# Supplementary material for: Evaluating Language Model Context Windows: A "Working Memory" Test and Inference-time Correction
Source: arXiv:2407.03651 source file (2024-07-14)
Supplement: Supplementary file 1 [file 1_glossary.tex]

\section{Glossary} \label{appendix:glossary}
\label{sec:gloss}
The glossary is given in Table~\ref{table:glossary} below.
\begin{table*}[h]
\centering
\begin{tabular}{l l}
\toprule
Symbol & Definition \\
\midrule
$\mathcal{X}$ & Feature space \\
$\mathcal{Y}$ & Label metric space\\
$\mathcal{Z}$ & Latent space of feature space \\
$A$ & Group variable, assumed to have one of two values \{0, 1\} for simplicity \\ 
$X_{k}$ & Inputs from group $k$.\\
$X$ & Inputs from all groups $k \in \{1, \ldots, l\}$\\
$Y_{k}$ & True labels from group $k$ \\
$Y$ & True labels from all groups $k \in \{1, \ldots, l\}$\\
$P$ & Probability distribution in the latent space\\
$P_k$ & Probability distribution in the group k\\

\multirow{2}{*}{$\lambda^{j}_{k}$} & Noisy labels of labeling function $j$ from group $k$. If it is used with input (e.g. $\lambda^{j}_{k}(x)$), \\
& it denotes labeling function $j$ from group $k$ such that its outputs are noisy labels\\
\multirow{2}{*}{$\lambda^{j}$} & Noisy labels of labeling function $j$ from all groups $k \in \{1, \ldots, l\}$. If it is used with input (e.g. $\lambda^{j}(x)$), \\
& it denotes labeling function $j$ such that its outputs are noisy labels\\
$\Lambda_{k}$ & Collection of noisy labels from group $k$, $\Lambda_{k} = [\lambda^1_{k}, \ldots, \lambda^{m}_{k}]$ \\
$\Lambda$ & Collection of noisy labels from all groups $k \in \{1, \ldots, l\}$, $\Lambda=[\lambda^{1}, \ldots, \lambda^{m}]$\\
$g_{k}$ & $g_{k}:\mathcal{Z} \to \mathcal{X}$, $k$-th group transformation function\\
$h_{k}$ & $h_{k}:\mathcal{X} \to \mathcal{Z}$ the inverse transformation of $g_k$, i.e. $h_{k}g_{k}(x)=x$ for $x \in \mathcal{Z}$\\
$\theta_{y}$ & Prior parameter for $Y$ in label model \\
$\theta_{j}$ & Accuracy parameter for $\lambda^{j}$ in label model \\ 
$\theta_{j, x}$ & Accuracy parameter for $x$ of $\lambda^{j}$ in label model \citep{chen2022shoring} \\ 
$a^{j}_{k}$ & Accuracy of LF $j$ in group $k$, $a^{j}_{k} = \E[\lambda_{j}Y|A=k]$\\
$a^{j}$ & Accuracy of LF $j$, $a^{j} = \E[\lambda_{j}Y]$\\
$\hat{a}^{j}_{k}, \hat{a}^{j}$ & Estimates of $a^{j}_{k}, a^{j}$ \\
$\mu_{k}$ & Mean of features in group $k$\\
$\Sigma_{k}$ & Covariance of features in group $k$\\
$I$ & Identity transformation, i.e. $I(x)=x$\\
$tr(\Sigma)$ & Trace of $\Sigma$ \\
$\lambda_{\max}(\Sigma), \lambda_{\min}(\Sigma)$ & Maximum, minimum values of $\Sigma$ \\

$\mathbf r(\Sigma)$ & Effective rank of $\Sigma$, i.e. $\mathbf r(\Sigma) = \frac{tr(\Sigma)}{\lambda_{\max}(\Sigma)}$\\
\toprule
\end{tabular}
\caption{
	Glossary of variables and symbols used in this paper.
}
\label{table:glossary}
\end{table*}
