# Supplementary material for: Evaluating Language Model Context Windows: A "Working Memory" Test and Inference-time Correction
Source: arXiv:2407.03651 source file (2024-07-14)
Supplement: Supplementary file 2 [file 2_more_backgrounds.tex]

\section{Extended related work} \label{appendix:more_backgrounds}
% Here we provide

\paragraph{Weak supervision}
In weak supervision, we assume true label $Y\in \mathcal{Y}$ cannot be accessed, but labeling functions $\lambda^{1}, \lambda^{2}, \cdots, \lambda^{m} \in \mathcal{Y}$ which are noisy versions of true labels, are given. These weak label sources include code snippets expressing heuristics about $Y$, crowdworkers, external knowledge bases, pretrained models, etc \citep{karger2011iterative, mintz2009distant, gupta2014improved, Dehghani2017, Ratner18}.
Given $\lambda^{1}, \lambda^{2}, \cdots, \lambda^{m}$, WS often takes a two-step procedure to get an end model \cite{dawid1979maximum, Ratner16, fu2020fast, ratner2019training, shin21universalizing, vishwakarmalifting}.
The first step is to get fine-grained pseudolabels by modeling accuracies and correlations of label sources.
The second step is training or fine-tuning the end model with pseudolabels to get better generalization than the label model.
Not only our method can improve performance and fairness, but also it is compatible with the previous WS label models since it works at the label source level before modeling the label model.

Another related line of works is WS using embeddings of inputs \cite{lang2022training, chen2022shoring}. \citet{lang2022training} uses embeddings for subset selection, where high-confidence subsets are selected based on the proximity to the same pseudolabels. \citet{chen2022shoring} exploits embedding to estimate local accuracy and improve coverage. Similarly, our method uses embedding to improve fairness by mapping points in different groups on the embedded space. Embedded space by a pre-trained model typically offers better distance metrics than the input space, which provides an advantage when the relationship between data points can be useful.

\paragraph{Fairness in machine learning}
Fairness in machine learning is an active research area to detect and address biases in ML algorithms. There have been many suggested fairness (bias) notions and solutions for them \cite{dwork2012fairness, hardt2016equality, kusner2017counterfactual, heidari2019long, gupta2019equalizing, huan2020fairness, guldogan2022equal}.
Popular approaches include adopting constrained optimization or regularization with fairness metrics \cite{dwork2012fairness, hardt2016equality, agarwal2018reductions, heidari2019long, gupta2019equalizing, huan2020fairness} and postprocessing model outputs to guarantee some fairness notions \cite{menon2018cost, zeng2022bayes}.
While they have been successful in reducing bias, those methods often have a fundamental tradeoff between accuracy and fairness.

A more recent line of works using Optimal Transport (OT) \cite{gordaliza2019obtaining, black2020fliptest, silvia2020general, si2021testing, buyl2022optimal} has shown that OT can be used to improve fairness without tradeoff by uniformizing distributions in different groups.
Our method improves fairness and performance spontaneously by utilizing OT.
However, OT-based methods can suffer from additional errors induced by optimal transport mapping.
In our method, OT-induced errors that occurred at the label sources can be covered by the label model, since worsened labeling functions would be down-weighted in label model fitting.
Our method has a limitation in the point that fairness scores after applying our methods are unpredictable in advance, while methods having fairness-accuracy tradeoff typically come with tunable parameters regarding the tradeoff.
However, as we argued in Section \ref{sec:experiment}, our method is compatible with other methods, thus it has the optionality to control the fairness of the end model by adopting other methods as well.
