# Supplementary material for: Evaluating Language Model Context Windows: A "Working Memory" Test and Inference-time Correction
Source: arXiv:2407.03651 source file (2024-07-14)
Supplement: Supplementary file 3 [file 3_algorithm_details.tex]

\section{Algorithm details} \label{appendix:algorithm-details}

\begin{figure}[!ht]
    \centering
        \includegraphics[width=\textwidth]{figures/overall_pipeline.pdf}
    \caption{Overall WS pipeline involving SBM}\label{fig:overall_pipeline}
\end{figure}

\begin{algorithm}[!ht]
    \caption{\textsc{Estimate Accuracy (Triplet) \citep{fu2020fast}}} \label{alg:triplet}
	\begin{algorithmic}
		\STATE \textbf{Parameters:}
        Weak label values $\lambda^{1}, \ldots, \lambda^{m}$

        \FOR{$i,j,k \in \{1,2,\ldots, m\}$ $(i\neq j \neq k)$}
        \STATE $|\hat{a}^{i}| \gets \sqrt{\hat{\mathbb{E}}[\lambda^i \lambda^j]\hat{\mathbb{E}}[\lambda^i \lambda^k]/\hat{\mathbb{E}}[\lambda^j \lambda^k]}$
        \STATE $|\hat{a}^{j}| \gets \sqrt{\hat{\mathbb{E}}[\lambda^i \lambda^j]\hat{\mathbb{E}}[\lambda^j \lambda^k]/\hat{\mathbb{E}}[\lambda^i\lambda^k]}$
        \STATE $|\hat{a}^{k}| \gets \sqrt{\hat{\mathbb{E}}[\lambda^i \lambda^k]\hat{\mathbb{E}}[\lambda^j \lambda^k]/\hat{\mathbb{E}}[\lambda^i \lambda^j]}$
        \ENDFOR

        \RETURN \text{ResolveSign} $(\hat{a}^{i}) \qquad \forall i \in \{1,2,\ldots, m\}$
  
	\end{algorithmic}
\end{algorithm}

\begin{algorithm}[!ht]
    \caption{\textsc{Transport}} \label{alg:transport}
	\begin{algorithmic}
		\STATE \textbf{Parameters:} Source input $X_{src}$, destination input $X_{dst}$, source weak label values $\lambda_{src}$, destination weak label values $\lambda_{dst}$, Optimal Transport type $O$, the number of nearest neighbors $k=1$
            \IF{OT type is linear}
            \STATE{$\tilde{X}_{src} \gets$ \textsc{LinearOT}$(X_{src}, X_{dst})$} \citep{knott1984optimal}
            \ELSIF{OT type is sinkhorn}
            \STATE{$\tilde{X}_{src} \gets$ \textsc{SinkhornOT}$(X_{src}, X_{dst})$} \citep{cuturi2013sinkhorn}
            \ELSE
            \STATE{$\tilde{X}_{src} \gets X_{src}$}
            \ENDIF
            \STATE{$\tilde{\lambda}_{src} \gets kNN(\tilde{X}_{src}, X_{dst}, \lambda_{dst}, k)$}
            \RETURN $\tilde{\lambda}_{src}$
	\end{algorithmic}

\end{algorithm}

\begin{algorithm}[!ht]
    \caption{\textsc{LinearOT}\cite{knott1984optimal}}\label{alg:linearOT}
	\begin{algorithmic}
		\STATE \textbf{Parameters:} Source input $X_{src}$, destination input $X_{dst}$        \STATE $\mu_{s}, \mu_{t} \gets \textsc{mean}(X_{src}), \textsc{mean}(X_{dst})$ 
            \STATE $\Sigma_{s}, \Sigma_{t} \gets \textsc{Cov}(X_{src}), \textsc{Cov}(X_{dst})$
            \STATE $A \gets \Sigma_{s}^{-1/2}(\Sigma_{s}^{1/2}\Sigma_{t}\Sigma_{s}^{1/2})^{1/2}\Sigma_{s}^{-1/2}$
            \STATE $b \gets \mu_t - A\mu_{s}$
            \STATE $B \gets [b \ \cdots \ b]$
            \STATE $\tilde{X}_{src} \gets X_{src}A^T + B^T$
            \RETURN $\tilde{X}_{src}$
	\end{algorithmic}
\end{algorithm}

\begin{algorithm}[!ht]
    \caption{\textsc{SinkhornOT}\cite{cuturi2013sinkhorn}}\label{alg:sinkhornOT}
	\begin{algorithmic}
		  \STATE \textbf{Parameters:} Source input $X_{src}$, destination input $X_{dst}$, Entropic regularization parameter $\eta$=1, max\_iter=10
            \STATE $M =\textsc{PairwiseDistance}(X_{src}, X_{dst})$

            \STATE $n_{src}, n_{dst} =  size(X_{src}), size(X_{dst})$
            \STATE $a, b = P(X_{src}), P(X_{dst})$
            \STATE $u, K, v = Sinkhorn(M, \eta, a, diag(b))$ // \textbf{Algorithm 1} of \cite{cuturi2013sinkhorn}
            \STATE $T = uKv^T$
            
            \STATE $\tilde{X}_{src} \gets T X_{dst}$ 
            \RETURN $\tilde{X}_{src}$
          
	\end{algorithmic}
\end{algorithm}

In this appendix section, we discuss the details of the algorithms we used. The overall WS pipeline including SBM is illustrated in Figure \ref{fig:overall_pipeline}. Our method is placed at the first step, as a refinement of noisy labels. In this step, we improve the noisy labels by transporting the low accuracy group to the high accuracy group. To identify low accuracy and high accuracy groups, we estimate accuracy using Algorithm \ref{alg:triplet}. After estimating accuracies, we transport the low accuracy group to the high accuracy group and get refined labels for the low accuracy group by Algorithm \ref{alg:transport}. Linear OT (Optimal Transport) is used to estimate a mapping. Sinkhorn OT approximates optimal coupling using Sinkhorn iteration. After obtaining the optimal coupling, data points from the low accuracy group are mapped to the coupled data points in the high accuracy group. If OT type is not given, data points from the low accuracy group are mapped to the 1-nearest neighbor in the high accuracy group. After obtaining mapped points, weak labels associated with mapped points in the target group are used for the data points from the low accuracy group.

The next step is a standard weak supervision pipeline step -- training a label model and running inference to obtain pseudolabels. Finally, we train the end model. We used the off-the-shelf label model Snorkel \citep{bach2018snorkel} for the label model and logistic regression as the end model in all experiments. For the optimal transport algorithm implementation, we used the Python POT package \citep{flamary2021pot}.

% \begin{algorithm}[H]
% \caption{Sinkhorn Optimal Transport}
% \begin{algorithmic}[1]
% \STATE Initialize $P = \frac{1}{nm} \mathbf{1}{n \times m}$
% \FOR{i=1 \text{ to max_iter}}
% \STATE $K = \frac{1}{a} \sum\limits{j=1}^m P_{:,j}$
% \STATE $P = P .* (K \times \mathbf{1}{1 \times m})$
% \STATE $L = \frac{1}{b} \sum\limits{i=1}^n P_{i,:}$
% \STATE $P = P .* (\mathbf{1}{n \times 1} \times L)$
% \IF{$\max{\left|\left|K.*a - \mathbf{1}\right|\right|{\infty}, \left|\left|L.*b - \mathbf{1}\right|\right|_{\infty}} < \epsilon$}
% \STATE \textbf{break}
% \ENDIF
% \ENDFOR
% \end{algorithmic}
% \end{algorithm}
