# Supplementary material for: Evaluating Language Model Context Windows: A "Working Memory" Test and Inference-time Correction
Source: arXiv:2407.03651 source file (2024-07-14)
Supplement: Supplementary file 4 [file 4_theory_details.tex]

\section{Theory details} \label{appendix:theory-details}

Accuracy is defined as $P(\lambda(x)=y)=P(\lambda(x)=1, y=1)+P(\lambda(x)=-1, y=-1)$. For ease of notation, below we set $\phi(x, x^{\text{center}_{0}}) = (1+||x - x^{\text{center}_{0}}||)^{-1}$.

\newtheorem*{T1}{Theorem~\ref{thrmUnfair}}

\newtheorem*{T2}{Theorem~\ref{thrmHhat}}

\subsection{Proof of Theorem~\ref{thrmUnfair}}

\begin{T1}
Let $g_1^{(k)}$ be an arbitrary sequence of functions such that $\lim_{k\to \infty} \mathbb E_{x' \in g_1^{(k)}(\mathcal X)} [||x'-x^{\text{center}_{0}}||] \rightarrow \infty$. %Furthermore, suppose that $\forall k, \forall \mathbf z \in \mathcal X$, $P(y| I(\mathbf z))=P(y| g^{(k)}(\mathbf z))$.
Suppose our assumptions above our met; in particular, that the label $y$ is independent of the observed features $x=I(z)$ or $x' =g_1^{(k)}(z), \forall k,$ conditioned on the latent features $z$. 
    Then, 
\[    \lim_{k \to \infty} \mathbb E_{x' \in g_1^{(k)}(\mathcal{Z})}[P(\lambda(x')= y)]= \frac{1}{2},\]
which corresponds to random guessing.
\end{T1}

\begin{proof}[Proof of Theorem~\ref{thrmUnfair}]
    Because $\lim_{k\to \infty} \mathbb E_{x' \in g_1^{(k)}(\mathcal{Z})} [||x'-x^{\text{center}_{0}}||]\to \infty$, we have 
    $$\lim_{k\to \infty} \mathbb E_{x' \in g_1^{(k)}(\mathcal{Z})} 
        [\phi(x', x^{\text{center}_{0}})] =0$$
        and because $Z=\sum_{i\in\{0,1\}} \sum_{j\in \{0,1\}} P(\lambda(x')=i, y=j)$,

\begin{align*}
    \lim_{k\to \infty} \mathbb E_{x' \in g_1^{(k)}(\mathcal{Z})} 
        [P(\lambda(x')=y)] &= \lim_{k\to \infty} \mathbb E_{x' \in g_1^{(k)}(\mathcal{Z})} \left[ P(\lambda(x')=1,y=1)+ P(\lambda(x')=-1, y=-1) \right]\\
        &= \lim_{k\to \infty} \mathbb E_{x' \in g_1^{(k)}(\mathcal{Z})} \left[\frac{1}{Z} \exp{(\theta_0 (1)(1) \phi(x', x^{\text{center}_{0}}) )} + \frac{1}{Z} \exp{(\theta_0 (-1)(-1) \phi(x', x^{\text{center}_{0}}) )}\right]\\
        &= \lim_{k\to \infty} \mathbb E_{x' \in g_1^{(k)}(\mathcal{Z})} \left[\frac{2}{Z} \exp{(\theta_0 \phi(x', x^{\text{center}_{0}}) )}\right]\\
        &= \lim_{k\to \infty} \mathbb E_{x' \in g_1^{(k)}(\mathcal{Z})} 
            \left[ \frac{2 \exp (\theta_0 \phi(x', x^{\text{center}_{0}}))}{2(\exp (\theta_0 \phi(x', x^{\text{center}_{0}})) + \exp (-\theta_0 \phi(x', x^{\text{center}_{0}})))} \right] \\
        &= \lim_{k\to \infty} \mathbb E_{x' \in g_1^{(k)}(\mathcal{Z})} 
            \left[ \frac{\exp (\theta_0 \phi(x', x^{\text{center}_{0}}))}{\exp (\theta_0 \phi(x', x^{\text{center}_{0}})) + \exp (-\theta_0 \phi(x', x^{\text{center}_{0}}))} \right] \\
        &=\frac{1}{2}.
\end{align*}
\end{proof}

\subsection{Proof of Theorem~\ref{thrmHhat}}

\begin{T2}
Let $\tau=\max \left(\frac{\mathbf r(\Sigma_0)}{n_0}, 
\frac{\mathbf r(\Sigma_1)}{n_1}, 
\frac{t}{\min(n_0,n_1)}, 
\frac{t^2}{\max(n_0,n_1)^2} \right)$ and $C$ be a constant. Using Algorithm~\ref{alg:sbm}, for any $t>0$, we bound the difference 

\begin{align*}
    |\mathbb E_{x \in \mathcal Z}[P(\lambda(x)=y)]-\mathbb E&_{x' \in \mathcal{X}} [P(\lambda(\hat h(x'))=y)]| \\
    &\leq 4\theta_0 C \sqrt{ \tau \mathbf r(\Sigma_1)}.
\end{align*}

with probability $1-e^{-t}-\frac{1}{n_1}$. 
\end{T2}

We use the result from \cite{flamary2019concentration}, which bounds the difference of the true $h$ and empirical $\hat h$ Monge estimators between two distributions $P_0(x)$ and $P_1(x')$. Let $\mathbf r(\Sigma)$, $\lambda_{\min}(\Sigma)$ and $\lambda_{\max}(\Sigma)$ denote the effective rank, minimum and maximum eigenvalues of matrix $\Sigma$ respectively. Then,

\begin{lemma}[\cite{flamary2019concentration}] \label{lem1}
Let $P_0(x)$ and $P_1(x')$ be sub-Gaussian distributions on $\mathcal X=\mathbb R^d$ with expectations $\mu_0, \mu_1$ and positive-definite covariance operators $\Sigma_0, \Sigma_1$ respectively. We observe $n_0$ points from the distribution $P_0(x)$ and $n_1$ points from the distribution $P_1(x')$. We assume that
\begin{equation*}
    c_1 < \min_{j\in \{0,1\}} \{\lambda_{\min}(\Sigma_j)\} \leq \max_{j\in \{0,1\}} \{\lambda_{\max} (\Sigma_j)\} \leq c_2,
\end{equation*}
for fixed constants $0 <c_1\leq c_2 < \infty$. Further, we assume $n_0\geq c \mathbf r(\Sigma_0)$ and $n_1 \geq d$ for sufficiently large constant $c>0$.

Then, for any $t>0$, we have with probability at least $1-e^{-t}-\frac{1}{n_1}$ that

\begin{equation*}
    \mathbb E_{x' \in \mathcal{X}} [|| h(x') - \hat h(x') ||] \leq C \sqrt{ \tau \mathbf r(\Sigma_1)},
\end{equation*}
where $C$ is a constant independent of $n_0, n_1, d, \mathbf r(\Sigma_0), \mathbf r(\Sigma_1)$ and $\tau=\max \left(\frac{\mathbf r(\Sigma_0)}{n_0}, 
\frac{\mathbf r(\Sigma_1)}{n_1}, 
\frac{t}{\min(n_0,n_1)}, 
\frac{t^2}{\max(n_0,n_1)^2} \right)$.
\end{lemma}
%\begin{proof}
%    See \cite{flamary2019concentration}.
%\end{proof}

We will also use the following:

\begin{lemma}\label{lemLipschitz}
    The probability $P(\lambda(x)=y)$ is $L$-Lipschitz with respect to $x \in \mathcal{X}$. Specifically, $\forall x_1, x_2 \in \mathcal X$,
    \begin{equation*}
        |P(\lambda(x_1)=y)-P(\lambda(x_2)=y)| \leq 4\theta_0 ||x_1-x_2||.
    \end{equation*}
\end{lemma}

\begin{proof}
    We will demonstrate that, because $||\nabla_{x} P(\lambda(x)=y)||$ is bounded above by $4\theta_0$, $P(\lambda(x)=y)$ must be $4\theta_0$-Lipschitsz with respect to $x$. First,
    \begin{align*}
        P(\lambda(x)=y) &= \frac{\exp(\theta_0 \phi(x, x^{\text{center}_{0}}))}{\exp(\theta_0 \phi(x, x^{\text{center}_{0}})) + \exp(-\theta_0 \phi(x, x^{\text{center}_{0}}))}\\
        &= \frac{1}{1+\exp(-2\theta_0 \phi(x, x^{\text{center}_{0}}))}\\
        &= \sigma(2\theta_0 \phi(x, x^{\text{center}_{0}})),
    \end{align*}
    where $\sigma$ denotes the sigmoid function. Note that $\frac{d}{d u} \sigma (u)=\frac{\exp(-u)}{(1+\exp(-u))^2}$ for $u\in \mathbb R$ and that $\nabla_{x} [2\theta_0 \phi(x, x^{\text{center}_{0}})] = 2 \theta_0 \nabla_{x} \left[ \frac{1}{1+||x-x^{\text{center}_{0}}||} \right] = 2 \theta_0 \frac{\nabla_{x} [||x-x^{\text{center}_{0}}||]}{(1+||x-x^{\text{center}_{0}}||)^2} $. Further, note that $\nabla_{x} [||x-x^{\text{center}_{0}}||]=\frac{x-x^{\text{center}_{0}}}{||x-x^{\text{center}_{0}}||}$ because we assume Euclidean norm. Thus,
    
    \begin{align*}
        ||\nabla_{x} P(\lambda(x)=y)|| &= ||\nabla_{x} \sigma (2\theta_0 \phi(x, x^{\text{center}_{0}}))||\\
        &= \left|\left| 2\theta_0  \frac{exp(-2\theta_0 \phi(x, x^{\text{center}_{0}}))}{(1+exp(-2\theta_0 \phi(x, x^{\text{center}_{0}})))^2(1+||x-x^{\text{center}_{0}}||)^2} \cdot \nabla_{x} [||x-x^{\text{center}_{0}}||]\right|\right| \\
        &= \left|\left| 2\theta_0  \frac{exp(-2\theta_0 \phi(x, x^{\text{center}_{0}}))}{(1+exp(-2\theta_0 \phi(x, x^{\text{center}_{0}})))^2} \phi(x, x^{\text{center}_{0}})^2 \cdot \frac{x-x^{\text{center}_{0}}}{||x-x^{\text{center}_{0}}||}\right|\right| \\
        &= \left|\left| 2\theta_0  \sigma(2\theta_0 \phi(x, x^{\text{center}_{0}}))(1-\sigma(2\theta_0 \phi(x, x^{\text{center}_{0}}))) \phi(x, x^{\text{center}_{0}})^2 \cdot \frac{x-x^{\text{center}_{0}}}{||x-x^{\text{center}_{0}}||} \right|\right|\\
        &< 2\theta_0 \left|\left|  1\cdot (1-(-1)) \phi(x, x^{\text{center}_{0}})^2 \cdot \frac{x-x^{\text{center}_{0}}}{||x-x^{\text{center}_{0}}||} \right|\right|\\
        &= 4\theta_0 \left|\left|  \phi(x, x^{\text{center}_{0}})^2 \cdot 1 \right|\right|\\
        &\leq 4\theta_0.
    \end{align*}

Thus, $||\nabla_{x} P(\lambda(x)=y)||$ is bounded above by $4\theta_0$. We now use this fact to demonstrate that $P(\lambda(x)=y)$ is $4\theta_0$-Lipschitz  with respect to $x$. 

% Because $||\nabla_{\mathbf x} P(\lambda(\mathbf x)=y)||\leq4\theta_0$, we have 
% \begin{align*}
%     \left|P(\lambda(\mathbf x_1)=y) - P(\lambda(\mathbf x_2)=y)\right| &=  \left| \int_{\mathbf x_1}^{\mathbf x_2} [\nabla_{\mathbf x} P(\lambda(\mathbf x)=y)] \nabla_{\mathbf x} \right| \\
%     &\leq  \int_{\mathbf x_1}^{\mathbf x_2} \left|| \nabla_{\mathbf x} P(\lambda(\mathbf x)=y) \right|| \nabla_{\mathbf x}  \\
%     &\leq \int_{\mathbf x_1}^{\mathbf x_2} 4\theta_0 \nabla_{\mathbf x}  \\
%     &= 4\theta_0 ||\mathbf x_1-\mathbf x_2||.
% \end{align*}

For $0\leq v\leq 1$, let $s(v)=x_1 + (x_2-x_1)v$. For $x$ between $x_1$ and $x_2$ inclusive and for $v$ such that $s(v)=x$, because $||\nabla_{x} P(\lambda(x)=y)||=|\frac{d}{dv}P(\lambda(s(v))=y)|\leq4\theta_0$, we have 
\begin{align*}
    \left|P(\lambda(x_1)=y) - P(\lambda(x_2)=y)\right| &=  \left| \int_{v=0}^{1} \left[\frac{d}{dv} P(\lambda(s(v))=y)\right] \space ||s(v)||dv \right| \\
    &\leq  \int_{v=0}^{1} \left|\frac{d}{dv} P(\lambda(s(v))=y)\right| \space ||s(v)||dv  \\
    &\leq \int_{v=0}^{1} 4\theta_0 ||s(v)||dv  \\
    &= 4\theta_0 ||x_1-x_2||.
\end{align*}

\end{proof}
% \hv{Are you using Mean value theorem above? how are you getting $||s(v)||$ in line 1?}

\begin{proof}[Proof of Theorem~\ref{thrmHhat}]
Now we are ready to complete our proof. We have,
\begin{align*}
|\mathbb E&_{x \in \mathcal Z}[P(\lambda(x)=y)]-\mathbb E_{x' \in \mathcal{X}} [P(\lambda(\hat h(x'))=y)]|\\
    &\leq \mathbb E_{z \in \mathcal{Z}} [|P(\lambda(I(z))=y) - P(\lambda(\hat h(g_1(z)))=y|]\\
    &=    \mathbb E_{z \in \mathcal{Z}} [|P(\lambda(h(g_1(z)))=y) - P(\lambda(\hat h(g_1(z)))=y|] \\
    &\leq \mathbb E_{z \in \mathcal{Z}} [4\theta_0|| h(g_1(z))-\hat h(g_1(z)) ||] \text{ (by Lemma~\ref{lemLipschitz})} \\
    &=\mathbb E_{x' \in \mathcal X} [4\theta_0|| h(x') - \hat h(x') ||]\\
    &\leq 4\theta_0 C \sqrt{ \tau \mathbf r(\Sigma_1)}, 
\end{align*}
where the last line holds with probability at least $1-e^{-t}-\frac{1}{n_1}$ by Lemma~\ref{lem1}.

\end{proof}

% Note that
% \begin{align*}
%     ||\nabla_{\mathbf x} P(\lambda(\mathbf x)=y)|| &= \sup_v \frac{||\nabla_{\mathbf x} v P(\lambda(\mathbf x)=y)||}{||v||}\\
%     &= \sup_v \lim_{\epsilon\to 0} \frac{|\epsilon| ||\nabla_{\mathbf x}v P(\lambda(\mathbf x)=y)|| }{|\epsilon| ||v||}\\
%     &= \sup_v \lim_{\epsilon\to 0} \frac{||\nabla_{\mathbf x} \epsilon v P(\lambda(\mathbf x)=y)||}{||\epsilon v||}\\
%     &\leq \sup_v \lim_{\epsilon\to 0} \frac{|| P(\lambda(\mathbf x + \epsilon v)=y)-P(\lambda(\mathbf x)=y)-\nabla_{\mathbf x}[\epsilon v P(\lambda(\mathbf x)=y)] ||}{||\epsilon v||} + \frac{||P(\lambda(\mathbf x+\epsilon v)=y)-P(\lambda(\mathbf x)=y)||}{||\epsilon v||}\\
%     &\leq \sup_v \lim_{\epsilon\to 0} \frac{|| P(\lambda(\mathbf x + \epsilon v)=y)-P(\lambda(\mathbf x)=y)-\nabla_{\mathbf x}[\epsilon v P(\lambda(\mathbf x)=y)] ||}{||\epsilon v||} + \frac{4\theta_0||\mathbf x+\epsilon v -\mathbf x||}{||\epsilon v||}\\
%     &=0 + 4\theta_0\\
%     &=4\theta_0.
% \end{align*}
