# Supplementary material for: Evaluating Language Model Context Windows: A "Working Memory" Test and Inference-time Correction
Source: arXiv:2407.03651 source file (2024-07-14)
Supplement: Supplementary file 5 [file 5_experiment_details.tex]

\section{Experiment details} \label{appendix:experiment-details}
\subsection{Dataset details}

\begin{table}[!ht]
    \centering
    \begin{tabular}{llll}
    \toprule
        & $P(Y=1|A=1)$ & $P(Y=1|A=0)$ & $\Delta_{DP}$ \\ \midrule
        Adult & 0.3038 & 0.1093 & 0.1945 \\ 
        Bank & 0.1093 & 0.2399 & 0.1306 \\ 
        CivilComments & 0.3154 & 0.1057 & 0.2097 \\ 
        HateXplain & 0.8040 & 0.4672 & 0.3368 \\ 
        CelebA & 0.3244 & 0.6590 & 0.3346 \\ 
        UTKFace & 0.4856 & 0.4610 & 0.0246 \\ \bottomrule
    \end{tabular}
    \caption{Distribution and inherent bias in datasets}
    \label{tab:data_fairness}
\end{table}

\paragraph{Adult} The adult dataset \citep{kohavi1996scaling} has information about the annual income of people and their demographics.
The classification task is to predict whether the annual income of a person exceeds \$50,000 based on demographic features.
Demographic features include age, work class, education, marital status, occupation, relationship, race, capital gain and loss, work hours per week, and native country.
The group variable is whether age is greater than 25 or not. The training data has 32561 examples, and the test data has 16281 examples.

\paragraph{BankMarketing} The bank marketing dataset \citep{moro2014data} was collected during the direct marketing campaigns of a Portuguese banking institution from 2008 to 2013.
Features consist of demographic attributes, financial attributes, and the attributes related to the interaction with the campaign.
The task is to classify whether a client will make a deposit subscription or not.
The group variable is, whether age is greater than 25 or not.
The total number of instances is 41188, where the training dataset has 28831 rows and the test dataset has 12357 rows.

\paragraph{CivilComments} The CivilComments dataset \citep{borkan2019nuanced} is constructed from data collected in Jigsaw online conversattion platform.
We used the dataset downloaded from \citep{koh2021wilds}.
Features are extracted using BERT \cite{devlin2018bert} embeddings from comments, and the task is to classify whether a given comment is toxic or not.
This dataset has annotations about the content type of comments, e.g. race, age, religion, etc.
We chose ``black'' as the group variable.
The total number of instances is 402820, where the training dataset has 269038 rows and the test dataset has 133782 rows.

\paragraph{HateXplain} The HateXplain dataset \citep{mathew2021hatexplain} is comments collected from Twitter and Gab and labeled through Amazon Mechanical Turk.
Features are extracted using BERT embeddings from comments.
The task is to classify whether a given comment is toxic or not.
This dataset has three label types - hate, offensive, or normal.
We used hate and offensive label types as ``toxic'' label, that is, if one of two labels types is 1 for a row, the row has label 1.
The dataset has annotations about the target communities - race, religion, gender, LGBTQ.
We used the race group as the group variable.
The total number of instances is 17281, where the training set has 15360 rows and the test set has 1921 rows.

\paragraph{CelebA} The CelebA dataset \citep{liu2015faceattributes} is the image datasets that has images of faces with various attributes.
Features are extracted using CLIP\citep{radford2021learning} embeddings from images.
We tried gender classification task from this dataset---various other tasks can be constructed.
We used ``Young'' as the group variable.
The total number of instances is 202599, where the training set has 162770 rows and the test set has 39829 rows.

\paragraph{UTKFace} UTKFace dataset \citep{zhifei2017cvpr} consists of faces images in the wild with annotations of age, gender, and ethnicity.
Features are extracted using CLIP embeddings from images.
This dataset has attributes of age, gender, race and we chose gender as label (Male:0, Female: 1), solving gender classification.
We used the race as the group variable, encoding ``Asian'' group as 1, other race groups as 0.
The total number of instances is 23705, where the training set has 18964 rows and the test set has 4741 rows.

\subsection{Application of LIFT} \label{appendix_subsec:lift} To use smooth embeddings in the transport step of tabular datasets (adult and bank marketing), we convert tabular data rows into text sentences and then get BERT embeddings.

\paragraph{Adult} First we decided r.pronoun for each row r from <r.sex> and then generated sentences with the following template. "<r.pronoun> is in her <r.age\_range>s. <r.pronoun> is from <r.nationality>. <r.pronoun> works in <r.workclass>. Specifically, <r.pronoun> has a <r.job> job. <r.pronoun> works <r.working\_hour> hours per week. <r.pronoun> total education year is <r.education\_years>. <r.pronoun> is <r.marital\_status>.  <r.pronoun> is <r.race>".

An example sentence is "She is in her 20s. She is from United-States. She works in private sector. Specifically, she has a sales job. She works 30 hours per week. Her total education year is 6 years. She is married. She is White."

\paragraph{Bank marketing} Similarly, text sentences for each row r are generated using the following template. "This person is <r.age> years old. This person works in a <r.job> job. This person is <r.marital\_status>. This person has a <r.education\_degree> degree. This person <if r.has\_housing\_loan "has" else "doesn't have"> a housing loan. This person <if r.has\_personal\_loan "has" else "doesn't have"> a personal loan. THis person's contact is <r.contact\_type>. The last contact was on <r.last\_contact\_weekday> in <r.last\_contact\_month>. The call lasted for <r.duration> seconds. <r.campaign> times of contacts performed during this campaign. Before this campaign, <r.previous> times of contacts have been performed for this person. The employment variation rate of this person is <r.emp\_var\_rate>\%. The consumer price index of this person is <r.cons\_price\_idx>\%. The consumer confidence index of this person is <r.cons\_conf\_idx>\%. The euribor 3 month rate of this person is <r.euribor3m>. The number of employees is <r.nr\_employed>".

An example sentence is "This person is 37 years old. This person works in a management job. This person is married. This person has a university degree. This person doesn't have a housing loan. This person has a personal loan. This person's contact is a cellular. The last contact was on a Thursday in May. The call lasted for 195 seconds. 1 times of contacts performed during this campaign. Before this campaign, 0 times of contacts have been performed for this person. The employment variation rate of this person is -1.8\%. The consumer price index of this person is 92.893\%. The consumer confidence index of this person is -46.2\%. The euribor 3 month rate of this person is 1.327\%. The number of employees is 5099."

\subsection{LF details} \label{appendix_subsec:lf_details}
In this subsection, we describe the labeling functions used in the experiments. The performances of labeling functions, including our SBM results, are reported in Table \ref{tab:tabular_LF} $\sim$ \ref{tab:vision_sinkhorn_LF}.

\paragraph{Adult} We generated heuristic labeling functions based on the features as follows.
\begin{itemize}
    \item LF 1 (age LF): True if the age is between 30 and 60. False otherwise.
    \item LF 2 (education LF): True if the person has a Bachelor, Master, PhD degree. False otherwise
    \item LF 3 (marital LF): True if marital status is married. False otherwise.
    \item LF 4 (relationship LF): True if relationship status is Wife, Own-child, or Husband, False otherwise.
    \item LF 5 (capital LF): True if the capital gain is >5000. False otherwise.
    \item LF 6 (race LF): True if Asian-Pac-Islander or race-Other. False otherwise.
    \item LF 7 (country LF): True if Germany, Japan, Greece, or China. False otherwise.
    \item LF 8 (workclass LF): True if the workclass is Self employed, federal government, local government, or state government. False otherwise.
    \item LF 9 (occupation LF): True if the occupation is sales, executive managerial, professional, or machine operator. False otherwise.
\end{itemize}

\paragraph{Bank marketing} Similar to Adult dataset, we generated heuristic labeling functions based on the features as follows.
\begin{itemize}
    \item LF 1 (loan LF): True if the person has loan previously.False otherwise.
    \item LF 2 (previous contact LF): True if the previous contact number is >1.1. False otherwise.
    \item LF 3 (duration LF): True if the duration of bank marketing phone call is > 6 min. False otherwise.
    \item LF 4 (marital LF): True if marital status is single. False otherwise.
    \item LF 5 (previous outcome LF): True if the previous campaign was successful. False otherwise.
    \item LF 6 (education LF): True if the education level is university degree or professional course taken. False otherwise.
\end{itemize}

\paragraph{CivilComments} We generated heuristic labeling functions based on the inclusion of specific word lists. If a comment has a word that is included in the word list of LF, it gets True for that LF.
\begin{itemize}
    \item LF 1 (sex LF): ["man", "men", "woman", "women", "male", "female",\
                 "guy", "boy", "girl", "daughter", "sex", "gender",\
                 "husband", "wife", "father", "mother", "rape", "mr.",\
                 "feminist", "feminism", "pregnant", "misogy", "pussy",\
                 "penis", "vagina", "butt", "dick"]
    \item LF 2 (LGBTQ LF): ["gay", "lesbian", "transgender", "homosexual",\
                 "homophobic", "heterosexual", "anti-gay", "same-sex",\
                 "bisexual", "biological"]
    \item LF 3 (religion LF): ["muslim", "catholic", "church", "christian", \
                 "god", "jesus", "christ", "jew", "islam", "israel",\
                 "bible", "bishop", "gospel", "clergy", "protestant", "islam"]
    \item LF 4 (race LF): ["white", "black", "racist", "trump",\
               "supremacist", "american", "canada", "kkk",\
               "nazi", "facist", "african", "non-white", "discrimination",\
               "hate", "neo-nazi", "asia", "china", "chinese"]
    \item LF 5 (toxic LF): ["crap", "damn", "bitch", "ass", "fuck", "bullshit", "hell", "jerk"]
    \item LF 6 (threat LF): ["shoot", "kill", "shot", "burn",\
                 "stab", "murder", "gun", "fire",\
                 "rape", "punch", "hurt", "hunt", "bullet", "hammer"] 
    \item LF 7 (insult LF): ["stupid", "idiot", "dumb", "liar",\
                 "poor", "disgusting", "moron", "nasty",\
                 "lack", "brain", "incompetent", "sociopath"]
\end{itemize}

\paragraph{HateXplain} We used heuristic the same labeling functions with CivilComments. However, their performance was close to random guess (accuracy close to 0.5), so we added 5 pretrained model LFs from detoxify \cite{Detoxify} repository. We used models listed as original, unbiased, multilingual, original-small, unbiased-small.

\paragraph{CelebA} We used models pretrained from other datasets as LFs.
\begin{itemize}
    \item LF 1: ResNet-18 fine-tuned on gender classification dataset \footnote{https://www.kaggle.com/datasets/cashutosh/gender-classification-dataset}
    \item LF 2: ResNet-34 fine-tuned on FairFace dataset
    \item LF 3: ResNet-34 fine-tuned on UTKFace dataset
    \item LF 4: ResNet-34 fine-tuned on UTKFace dataset (White only)
    \item LF 5: ResNet-34 fine-tuned on UTKFace dataset (non-White only)
    \item LF 6: ResNet-34 fine-tuned on UTKFace dataset (age $\geq 50$ only)
    \item LF 7: ResNet-34 fine-tuned on UTKFace dataset (age $< 50$ only)
\end{itemize}

\paragraph{UTKFace} We used models pretrained from other datasets as LFs.
\begin{itemize}
    \item LF 1: ResNet-18 fine-tuned on gender classification dataset 
    \item LF 2: ResNet-34 fine-tuned on gender classification dataset 
    \item LF 3: ResNet-34 fine-tuned on CelebA dataset
    \item LF 4: ResNet-34 fine-tuned on CelebA dataset (attractive only)
    \item LF 5: ResNet-34 fine-tuned on CelebA dataset (non-attractive only)
    \item LF 6: ResNet-34 fine-tuned on CelebA dataset (young only)
    \item LF 7: ResNet-34 fine-tuned on CelebA dataset (non-young only)
    \item LF 8: ResNet-34 fine-tuned on CelebA dataset (unfair sampling)
\end{itemize}

\begin{table}
\caption{Tabular dataset raw LF performance}
   \label{tab:tabular_LF}
   \centering
   \begin{tabular}{llllll}
     \toprule
    Dataset & LF & Acc & F1 & $\Delta_{DP}$ & $\Delta_{EO} $  \\
     \midrule
     \multirow{5}{*}{Adult} & LF 1 (age LF) & 0.549 & 0.476 & 0.100 & 0.023 \\
                            & LF 2 (education LF) & 0.743 & 0.455 & 0.033 & 0.044 \\
                            & LF 3 (marital LF) & 0.699 & 0.579 & 0.447 & 0.241 \\
                            & LF 4 (relationship LF) & 0.564 & 0.486 & 0.381 & 0.243 \\
                            & LF 5 (capital LF) & 0.800 & 0.315 & 0.035 & 0.019 \\
                            & LF 6 (race LF) & 0.737 & 0.066 & 0.003 & 0.004 \\
                            & LF 7 (country LF) & 0.756 & 0.024 & 0.001 & 0.004 \\
                            & LF 8 (workclass LF) & 0.678 & 0.399 & 0.066 & 0.003 \\
                            & LF 9 (occupation LF) & 0.644 & 0.466 & 0.013 & 0.012 \\
     \midrule
     \multirow{5}{*}{Bank Marketing} & LF 1 (loan LF) & 0.769 & 0.124 & 0.004 & 0.013 \\
                            & LF 2 (previous contact LF) & 0.888 & 0.187 & 0.055 & 0.068 \\
                            & LF 3 (duration LF) & 0.815 & 0.415 & 0.019 & 0.125 \\
                            & LF 4 (marital LF): & 0.682 & 0.197 & 0.602 & 0.643 \\
                            & LF 5 (previous outcome LF) & 0.898 & 0.301 & 0.052 & 0.062 \\
                            & LF 6 (education LF) & 0.575 & 0.206 & 0.183 & 0.219 \\
    \bottomrule
   \end{tabular}
 \end{table}

\begin{table} \label{tab:tabular_naive_LF}

\caption{Tabular dataset SBM (w/o OT) LF performance. $\Delta$s are obtained by comparison with raw LF performance.}

    \centering
    \begin{tabular}{llllllll}
    \toprule
        Dataset & LF & Acc ($\Delta$) & F1 ($\Delta$) & $\Delta_{DP}$ ($\Delta$) & $\Delta_{EO}$ ($\Delta$) \\
        \midrule 
        \multirow{5}{*}{Adult} &
        LF 1 & 0.597 (0.048) & 0.594 (0.118) & 0.119 (0.019) & 0.106 (0.083) \\ 
        & LF 2 & 0.601 (-0.142) & 0.346 (-0.109) & 0.035 (0.002) & 0.019 (-0.025) \\
        & LF 3 & 0.998 (0.299) & 0.998 (0.419) & 0.303 (-0.144) & 0.001 (-0.240) \\ 
        & LF 4 & 0.719 (0.155) & 0.723 (0.237) & 0.304 (-0.077) & 0.091 (-0.152) \\ 
        & LF 5 & 0.649 (-0.151) & 0.183 (-0.132) & 0.035 (0.000) & 0.023 (0.004) \\ 
        & LF 6 & 0.615 (-0.122) & 0.082 (0.016) & 0.003 (0.000) & 0.029 (0.025) \\ 
        & LF 7 & 0.621 (-0.135) & 0.023 (-0.001) & 0.001 (0.000) & 0.005 (0.001) \\ 
        & LF 8 & 0.612 (-0.066) & 0.318 (-0.021) & 0.019 (-0.047) & 0.027 (0.024) \\
        & LF 9 & 0.565 (-0.079) & 0.460 (-0.006) & 0.013 (0.000) & 0.026 (0.014) \\ 
        \midrule
        \multirow{5}{*}{Adult (LIFT)} & LF 1 & 0.506 (-0.043) & 0.415 (-0.061) & 0.309 (0.209) & 0.198 (0.175) \\
        & LF 2 & 0.861 (0.118) & 0.691 (0.236) & 0.080 (0.047) & 0.126 (0.082) \\
        & LF 3 & 0.691 (-0.008) & 0.188 (-0.391) & 0.130 (-0.317) & 0.186 (-0.055) \\
        & LF 4 & 0.391 (-0.173) & 0.307 (-0.179) & 0.455 (0.074) & 0.314 (0.071) \\
        & LF 5 & 0.725 (-0.075) & 0.117 (-0.198) & 0.014 (-0.021) & 0.029 (0.010) \\
        & LF 6 & 0.703 (-0.034) & 0.109 (0.043) & 0.003 (0.000) & 0.004 (0.000) \\
        & LF 7 & 0.708 (-0.048) & 0.036 (0.012) & 0.001 (0.000) & 0.000 (-0.004) \\
        & LF 8 & 0.897 (0.219) & 0.800 (0.461) & 0.033 (-0.033) & 0.235 (0.232) \\
        & LF 9 & 0.601 (-0.043) & 0.446 (-0.020) & 0.013 (0.000) & 0.068 (0.056) \\ 
        \midrule
        \multirow{5}{*}{Bank} & LF 1 & 0.706 (-0.063) & 0.165 (0.041) & 0.004 (0.000) & 0.003 (-0.010) \\
        & LF 2 & 0.824 (-0.064) & 0.221 (0.034) & 0.037 (-0.018) & 0.113 (0.045) \\ 
        & LF 3 & 0.931 (0.116) & 0.829 (0.414) & 0.019 (0.000) & 0.110 (-0.015) \\ 
        & LF 4 & 0.427 (-0.255) & 0.411 (0.214) & 0.100 (-0.502) & 0.004 (-0.639) \\
        & LF 5 & 0.833 (-0.065) & 0.287 (-0.014)& 0.061 (0.009) & 0.195 (0.133) \\ 
        & LF 6 & 0.624 (0.049) & 0.172 (-0.034) & 0.009 (-0.174) & 0.046 (-0.173) \\
        \midrule
        \multirow{5}{*}{Bank (LIFT)} & LF 1 & 0.768 (-0.001) & 0.105 (-0.019) & 0.000 (-0.003) & 0.013 (0.000) \\ 
        & LF 2 & 0.888 (0.000) & 0.188 (0.001) & 0.037 (-0.017) & 0.068 (0.000)\\
        & LF 3 & 0.815 (0.000) & 0.415 (0.000) & 0.019 (0.000) & 0.125 (0.000) \\
        & LF 4 & 0.317 (-0.365) & 0.228 (0.031) & 0.100 (-0.502) & 0.065 (-0.578) \\
        & LF 5 & 0.898 (0.000) & 0.303 (0.001) & 0.061 (0.009) & 0.086 (0.023) \\ 
        & LF 6 & 0.680 (0.105) & 0.126 (-0.081) & 0.009 (-0.175) & 0.084 (-0.134) \\ 
    \bottomrule
    \end{tabular}
\end{table}

\begin{table}

\label{tab:tabular_linear_LF}
\caption{Tabular dataset SBM (OT linear) LF performance. $\Delta$s are obtained by comparison with raw LF performance.}
    \centering
    \begin{tabular}{llllllll}
    \toprule
    Dataset & LF & Acc ($\Delta$) & F1 ($\Delta$) & $\Delta_{DP}$ ($\Delta$) & $\Delta_{EO}$ ($\Delta$) \\ 
    \midrule
    \multirow{5}{*}{Adult} & LF 1 & 0.841 (0.292) & 0.846 (0.370) & 0.654 (0.554) & 0.733 (0.710) \\
    & LF 2 & 0.334 (-0.409) & 0.000 (-0.455) & 0.208 (0.175) & 0.000 (-0.044) \\
    & LF 3 & 0.346 (-0.353) & 0.000 (-0.579) & 0.174 (-0.273) & 0.000 (-0.241) \\ 
    & LF 4 & 0.895 (0.331) & 0.904 (0.418) & 0.735 (0.354) & 0.824 (0.581) \\ 
    & LF 5 & 0.394 (-0.406) & 0.000 (-0.315) & 0.027 (-0.008) & 0.000 (-0.019) \\ 
    & LF 6 & 0.408 (-0.329) & 0.070 (0.004) & 0.003 (0.000) & 0.037 (0.033) \\
    & LF 7 & 0.405 (-0.351) & 0.019 (-0.005) & 0.001 (0.000) & 0.010 (0.006) \\
    & LF 8 & 0.336 (-0.342) & 0.000 (-0.339) & 0.202 (0.136) & 0.000 (-0.003) \\
    & LF 9 & 0.501 (-0.143) & 0.512 (0.046) & 0.013 (0.000) & 0.439 (0.427) \\
    \midrule
    \multirow{5}{*}{Adult (LIFT)} & LF 1 & 0.628 (0.079) & 0.655 (0.179) & 0.036 (-0.064) & 0.027 (0.004) \\ 
    & LF 2 & 0.780 (0.037) & 0.664 (0.209) & 0.014 (-0.019) & 0.032 (-0.012) \\ 
    & LF 3 & 0.525 (-0.174) & 0.296 (-0.283)  & 0.097 (-0.350) & 0.013 (-0.228) \\ 
    & LF 4 & 0.497 (-0.067) & 0.554 (0.068)  & 0.137 (-0.244) & 0.150 (-0.093) \\ 
    & LF 5 & 0.606 (-0.194) & 0.177 (-0.138) & 0.023 (-0.012) & 0.042 (0.023) \\ 
    & LF 6 & 0.565 (-0.172) & 0.089 (0.023) & 0.003 (0.000) & 0.008 (0.004) \\ 
    & LF 7 & 0.567 (-0.189) & 0.029 (0.005) & 0.001 (0.000) & 0.000 (-0.004) \\
    & LF 8 & 0.618 (-0.060) & 0.409 (0.070) & 0.011 (-0.055) & 0.017 (0.014) \\
    & LF 9 & 0.843 (0.199) & 0.817 (0.351) & 0.013 (0.000) & 0.046 (0.034) \\ 
    \midrule
    \multirow{5}{*}{Bank} & LF 1 & 0.818 (0.049) & 0.062 (-0.062) & 0.004 (0.000) & 0.140 (0.127) \\ 
    & LF 2 & 0.980 (0.092) & 0.703 (0.516)  & 0.024 (-0.031) & 0.542 (0.474) \\ 
    & LF 3 & 0.777 (-0.038) & 0.093 (-0.322)& 0.019 (0.000) & 0.265 (0.139) \\
    & LF 4 & 0.047 (-0.635) & 0.083 (-0.114) & 0.131 (-0.471) & 1.000 (0.357) \\
    & LF 5 & 0.988 (0.090) & 0.839 (0.538)  & 0.032 (-0.020) & 0.723 (0.660) \\
    & LF 6 & 0.950 (0.375) & 0.000 (-0.206) & 0.244 (0.061) & 0.000 (-0.219) \\
    \midrule
    \multirow{5}{*}{Bank (LIFT)} & LF 1 & 0.125 (-0.645) & 0.197 (0.073) & 0.853 (0.849) & 0.867 (0.854) \\
    & LF 2 & 0.888 (0.000) & 0.180 (-0.007) & 0.000 (-0.055) & 0.036 (-0.032) \\
    & LF 3 & 0.815 (0.000) & 0.415 (0.000) & 0.018 (-0.001) & 0.137 (0.012) \\
    & LF 4 & 0.876 (0.194) & 0.085 (-0.112) & 0.869 (0.268) & 0.954 (0.311) \\
    & LF 5 & 0.898 (0.000) & 0.300 (-0.002) & 0.047 (-0.005) & 0.039 (-0.023) \\
    & LF 6 & 0.124 (-0.451) & 0.198 (-0.008) & 0.756 (0.572) & 0.717 (0.498) \\
    \bottomrule
    \end{tabular}
\end{table}

\begin{table}

\label{tab:tabular_sinkhorn_LF}
\caption{Tabular dataset SBM (OT sinkhorn) LF performance. $\Delta$s are obtained by comparison with raw LF performance.}
    \centering
    \begin{tabular}{llllll}
    \toprule
        Dataset & LF & Acc ($\Delta$) & F1 ($\Delta$) & $\Delta_{DP}$ ($\Delta$) & $\Delta_{EO}$ ($\Delta$) \\ 
        \midrule
        \multirow{5}{*}{Adult} & LF 1 & 0.604 (0.055) & 0.595 (0.119) & 0.145 (0.045) & 0.125 (0.102) \\ 
        & LF 2 & 0.601 (-0.142) & 0.340 (-0.115) & 0.036 (0.003) & 0.015 (-0.029) \\
        &LF 3 & 0.998 (0.299) & 0.998 (0.419) & 0.293 (-0.154) & 0.002 (-0.239) \\ 
        &LF 4 & 0.690 (0.126) & 0.700 (0.214) & 0.221 (-0.160) & 0.050 (-0.193) \\ 
        &LF 5 & 0.656 (-0.144) & 0.181 (-0.134) & 0.032 (-0.003) & 0.021 (0.002) \\ 
        &LF 6 & 0.621 (-0.116) & 0.081 (0.015) & 0.003 (0.000) & 0.030 (0.026) \\ 
        &LF 7 & 0.627 (-0.129) & 0.023 (-0.001) & 0.001 (0.000) & 0.005 (0.001) \\ 
        &LF 8 & 0.607 (-0.071) & 0.256 (-0.083) & 0.069 (0.003) & 0.095 (0.092) \\ 
        &LF 9 & 0.558 (-0.086) & 0.446 (-0.020) & 0.013 (0.000) & 0.014 (0.002) \\
        \midrule
        \multirow{5}{*}{Adult (LIFT)} &LF 1 & 0.475 (-0.074) & 0.436 (-0.040) & 0.031 (-0.069) & 0.032 (0.009) \\ 
        &LF 2 & 0.953 (0.210) & 0.910 (0.455) & 0.047 (0.014) & 0.079 (0.035) \\ 
        &LF 3 & 0.712 (0.013) & 0.191 (-0.388) & 0.157 (-0.290) & 0.250 (0.009) \\ 
        &LF 4 & 0.373 (-0.191) & 0.425 (-0.061) & 0.204 (-0.177) & 0.120 (-0.123) \\
        &LF 5 & 0.764 (-0.036) & 0.301 (-0.014) & 0.035 (0.000) & 0.107 (0.088) \\ 
        &LF 6 & 0.711 (-0.026) & 0.117 (0.051) & 0.003 (0.000) & 0.018 (0.014) \\ 
        &LF 7 & 0.715 (-0.041) & 0.037 (0.013) & 0.001 (0.000) & 0.002 (-0.002) \\ 
        &LF 8 & 0.716 (0.038) & 0.272 (-0.067) & 0.147 (0.081) & 0.284 (0.281) \\ 
        &LF 9 & 0.640 (-0.004) & 0.495 (0.029) & 0.013 (0.000) & 0.213 (0.201) \\ 
        \midrule
        \multirow{5}{*}{Bank} &LF 1 & 0.694 (-0.075) & 0.173 (0.049) & 0.004 (0.000) & 0.017 (0.004) \\ 
        &LF 2 & 0.806 (-0.082) & 0.209 (0.022) & 0.059 (0.004) & 0.211 (0.143) \\ 
        &LF 3 & 0.949 (0.134) & 0.881 (0.466) & 0.019 (0.000) & 0.136 (0.011) \\ 
        &LF 4 & 0.351 (-0.331) & 0.382 (0.185) & 0.040 (-0.562) & 0.016 (-0.627) \\ 
        &LF 5 & 0.814 (-0.084) & 0.267 (-0.034) & 0.069 (0.017) & 0.247 (0.185) \\ 
        &LF 6 & 0.583 (0.008) & 0.020 (-0.186) & 0.040 (-0.143) & 0.103 (-0.116) \\
        \midrule
        \multirow{5}{*}{Bank (LIFT)} & LF 1 & 0.769(-0.001) & 0.087 (-0.038) & 0.006 (0.003) & 0.038 (0.025)\\ 
        &LF 2 & 0.888 (0.001) & 0.204 (0.017) & 0.141 (0.087) & 0.305 (0.237) \\
        &LF 3 & 0.814 (-0.001) & 0.409 (-0.006) & 0.054 (0.035) & 0.357 (0.231) \\ 
        &LF 4 & 0.307 (-0.375) & 0.229 (0.032) & 0.085 (-0.517) & 0.042 (-0.600) \\ 
        &LF 5 & 0.898 (0.000) & 0.311 (0.010) & 0.133 (0.081) & 0.236 (0.173) \\
        &LF 6 & 0.677 (0.102) & 0.105 (-0.102) & 0.003 (-0.180) & 0.122 (-0.096) \\ 
    \bottomrule
    \end{tabular}
\end{table}

\begin{table}

\caption{NLP dataset raw LF performance}
   \label{tab:NLP_LF}
   \centering
   \begin{tabular}{llllll}
     \toprule
    Dataset & LF & Acc & F1 & $\Delta_{DP}$ & $\Delta_{EO} $  \\
     \midrule
     \multirow{5}{*}{CivilComments} & LF 1 (sex LF) & 0.755 & 0.187 & 0.046 & 0.019 \\
                            & LF 2 (LGBTQ LF) & 0.877 & 0.073 & 0.001 & 0.017 \\
                            & LF 3 (religion LF) & 0.861 & 0.049 & 0.012 & 0.013 \\
                            & LF 4 (race LF) & 0.847 & 0.234 & 0.634 & 0.574 \\
                            & LF 5 (toxic LF) & 0.886 & 0.068 & 0.006 & 0.012 \\
                            & LF 6 (threat LF) & 0.862 & 0.102 & 0.055 & 0.054 \\
                            & LF 7 (insult LF) & 0.872 & 0.176 & 0.028 & 0.035 \\
     \midrule
     \multirow{5}{*}{HateXplain} & LF 1 (sex LF) & 0.427 & 0.253 & 0.015 & 0.002 \\
                            & LF 2 (LGBTQ LF) & 0.405 & 0.077 & 0.047 & 0.041 \\
                            & LF 3 (religion LF) & 0.437 & 0.197 & 0.001 & 0.003 \\
                            & LF 4 (race LF) & 0.419 & 0.327 & 0.139 & 0.168 \\
                            & LF 5 (toxic LF) & 0.451 & 0.233 & 0.007 & 0.016 \\
                            & LF 6 (threat LF) & 0.415 & 0.097 & 0.000 & 0.004 \\
                            & LF 7 (insult LF) & 0.427 & 0.100 & 0.015 & 0.005 \\
                            & LF 8 (Detoxify - original) & 0.645 & 0.704 & 0.165 & 0.086 \\
                            & LF 9 (Detoxify - unbiased) & 0.625 & 0.668 & 0.150 & 0.078 \\
                            & LF 10 (Detoxify - multilingual) & 0.649 & 0.700 & 0.168 & 0.077 \\
                            & LF 11 (Detoxify - original-small) & 0.644 & 0.705 & 0.152 & 0.076 \\
                            & LF 12 (Detoxify - unbiased-small) & 0.643 & 0.699 & 0.186 & 0.113 \\
    \bottomrule
   \end{tabular}
 \end{table}

\begin{table}

\label{tab:nlp_naive_LF}
\caption{NLP dataset SBM (w/o OT) LF performance. $\Delta$s are obtained by comparison with raw LF performance.}
    \centering
    \begin{tabular}{llllll}
    \toprule
        Dataset & LF & Acc ($\Delta$) & F1 ($\Delta$) & $\Delta_{DP}$ ($\Delta$) & $\Delta_{EO}$ ($\Delta$) \\ 
        \midrule
        \multirow{5}{*}{Civil Comments} & LF 1 & 0.790 (0.035) & 0.325 (0.138) & 0.048 (0.002) & 0.041 (0.022) \\
        &LF 2 & 0.896 (0.019) & 0.268 (0.195) & 0.001 (0.000) & 0.053 (0.036) \\ 
        &LF 3 & 0.868 (0.007) & 0.155 (0.106) & 0.012 (0.000) & 0.043 (0.030) \\ 
        &LF 4 & 0.858 (0.011) & 0.252 (0.018) & 0.114 (-0.520) & 0.160 (-0.414) \\ 
        &LF 5 & 0.886 (0.000) & 0.137 (0.069) & 0.006 (0.000) & 0.003 (-0.009) \\ 
        &LF 6 & 0.916 (0.054) & 0.482 (0.380) & 0.023 (-0.032) & 0.002 (-0.052) \\ 
        &LF 7 & 0.918 (0.046) & 0.501 (0.325) & 0.022 (-0.006) & 0.012 (-0.023) \\ 
        \midrule
        \multirow{5}{*}{HateXplain} & LF 1 & 0.483 (0.056) & 0.273 (0.020) & 0.015 (0.000) & 0.001 (-0.001) \\
        &LF 2 & 0.473 (0.068) & 0.058 (-0.019) & 0.000 (-0.047) & 0.004 (-0.037) \\ 
        &LF 3 & 0.460 (0.023) & 0.163 (-0.034) & 0.001 (0.000) & 0.004 (0.001) \\ 
        &LF 4 & 0.481 (0.062) & 0.328 (0.001) & 0.044 (-0.095) & 0.039 (-0.129) \\ 
        &LF 5 & 0.515 (0.064) & 0.267 (0.034) & 0.014 (0.007) & 0.021 (0.005) \\ 
        &LF 6 & 0.471 (0.056) & 0.106 (0.009) & 0.000 (0.000) & 0.015 (0.011) \\ 
        &LF 7 & 0.472 (0.045) & 0.088 (-0.012) & 0.012 (-0.003) & 0.014 (0.009) \\ 
        &LF 8 & 0.831 (0.186) & 0.864 (0.160) & 0.006 (-0.159) & 0.000 (-0.086) \\ 
        &LF 9 & 0.917 (0.292) & 0.928 (0.260) & 0.015 (-0.135) & 0.000 (-0.078) \\ 
        &LF 10 & 0.864 (0.215) & 0.888 (0.188) & 0.009 (-0.159) & 0.000 (-0.077) \\ 
        &LF 11 & 0.839 (0.195) & 0.870 (0.165) & 0.015 (-0.137) & 0.000 (-0.076) \\ 
        &LF 12 & 0.837 (0.194) & 0.868 (0.169) & 0.014 (-0.172) & 0.000 (-0.113) \\ 
        \bottomrule
    \end{tabular}
\end{table}

\begin{table}

\label{tab:nlp_linear_LF}
\caption{NLP dataset SBM (OT linear) LF performance. $\Delta$s are obtained by comparison with raw LF performance.}
    \centering
    \begin{tabular}{llllll}
    \toprule
        Dataset & LF & Acc ($\Delta$) & F1 ($\Delta$) & $\Delta_{DP}$ ($\Delta$) & $\Delta_{EO}$ ($\Delta$) \\ 
        \midrule
        \multirow{5}{*}{Civil Comments} & LF 1 & 0.791 (0.036) & 0.321 (0.134) & 0.003 (-0.043) & 0.022 (0.003) \\
        &LF 2 & 0.898 (0.021) & 0.272 (0.199) & 0.001 (0.000) & 0.020 (0.003) \\ 
        &LF 3 & 0.870 (0.009) & 0.156 (0.107) & 0.012 (0.000) & 0.041 (0.028) \\ 
        &LF 4 & 0.860 (0.013) & 0.244 (0.010) & 0.017 (-0.617) & 0.017 (-0.557) \\ 
        &LF 5 & 0.887 (0.001) & 0.139 (0.071) & 0.006 (0.000) & 0.027 (0.015) \\ 
        &LF 6 & 0.917 (0.055) & 0.484 (0.382) & 0.012 (-0.043) & 0.026 (-0.028) \\ 
        &LF 7 & 0.919 (0.047) & 0.501 (0.325) & 0.007 (-0.021) & 0.013 (-0.022) \\ 
        \midrule
        \multirow{5}{*}{HateXplain} & LF 1 & 0.457 (0.030) & 0.279 (0.026) & 0.015 (0.000) & 0.001 (-0.001) \\
        &LF 2 & 0.433 (0.028) & 0.062 (-0.015) & 0.002 (-0.045) & 0.006 (-0.035) \\ 
        &LF 3 & 0.429 (-0.008) & 0.171 (-0.026) & 0.001 (0.000) & 0.001 (-0.002) \\ 
        &LF 4 & 0.457 (0.038) & 0.323 (-0.004) & 0.011 (-0.128) & 0.009 (-0.159) \\ 
        &LF 5 & 0.479 (0.028) & 0.263 (0.030) & 0.017 (0.010) & 0.029 (0.013) \\ 
        &LF 6 & 0.436 (0.021) & 0.111 (0.014) & 0.000 (0.000) & 0.011 (0.007) \\ 
        &LF 7 & 0.434 (0.007) & 0.091 (-0.009) & 0.012 (-0.003) & 0.017 (0.012) \\
        &LF 8 & 0.845 (0.200) & 0.882 (0.178) & 0.790 (0.093) & 0.000 (-0.086) \\ 
        &LF 9 & 0.923 (0.298) & 0.938 (0.270) & 0.883 (0.179) & 0.000 (-0.078) \\ 
        &LF 10 & 0.875 (0.226) & 0.903 (0.203) & 0.823 (0.111) & 0.000 (-0.077) \\
        &LF 11 & 0.848 (0.204) & 0.884 (0.179) & 0.792 (0.098) & 0.000 (-0.076) \\
        &LF 12 & 0.845 (0.202) & 0.882 (0.183) & 0.789 (0.090) & 0.000 (-0.113) \\
        \bottomrule
    \end{tabular}
\end{table}

\begin{table}

\label{tab:nlp_sinkhorn_LF}
\caption{NLP dataset SBM (OT sinkhorn) LF performance. $\Delta$s are obtained by comparison with raw LF performance.}
    \centering
    \begin{tabular}{llllll}
    \toprule
        Dataset & LF & Acc ($\Delta$) & F1 ($\Delta$) & $\Delta_{DP}$ ($\Delta$) & $\Delta_{EO}$ ($\Delta$) \\ 
        \midrule
        \multirow{5}{*}{Civil Comments} &LF 1 & 0.791 (0.036) & 0.320 (0.133) & 0.015 (-0.031) & 0.082 (0.063) \\
        &LF 2 & 0.897 (0.020) & 0.271 (0.198) & 0.001 (0.000) & 0.029 (0.012) \\ 
        &LF 3 & 0.870 (0.009) & 0.156 (0.107) & 0.012 (0.000) & 0.043 (0.030) \\ 
        &LF 4 & 0.860 (0.013) & 0.245 (0.011) & 0.017 (-0.617) & 0.016 (-0.558) \\
        &LF 5 & 0.887 (0.001) & 0.138 (0.070) & 0.006 (0.000) & 0.020 (0.008) \\ 
        &LF 6 & 0.917 (0.055) & 0.482 (0.380) & 0.011 (-0.044) & 0.006 (-0.048) \\
        &LF 7 & 0.919 (0.047) & 0.504 (0.328) & 0.019 (-0.009) & 0.039 (0.004) \\ 
        \midrule
        \multirow{5}{*}{HateXplain} & LF 1 & 0.444 (0.017) & 0.277 (0.024) & 0.015 (0.000) & 0.002 (0.000) \\
        &LF 2 & 0.417 (0.012) & 0.056 (-0.021) & 0.001 (-0.046) & 0.001 (-0.040) \\
        &LF 3 & 0.418 (-0.019) & 0.172 (-0.025) & 0.001 (0.000) & 0.002 (-0.001) \\
        &LF 4 & 0.448 (0.029) & 0.332 (0.005) & 0.032 (-0.107) & 0.045 (-0.123) \\
        &LF 5 & 0.459 (0.008) & 0.256 (0.023) & 0.030 (0.023) & 0.041 (0.025) \\ 
        &LF 6 & 0.422 (0.007) & 0.110 (0.013) & 0.000 (0.000) & 0.011 (0.007) \\ 
        &LF 7 & 0.418 (-0.009) & 0.091 (-0.009) & 0.018 (0.003) & 0.025 (0.020) \\
        &LF 8 & 0.851 (0.206) & 0.889 (0.185) & 0.056 (-0.109) & 0.000 (-0.086) \\
        &LF 9 & 0.927 (0.302) & 0.942 (0.274) & 0.061 (-0.089) & 0.000 (-0.078) \\
        &LF 10 & 0.884 (0.235) & 0.911 (0.211) & 0.052 (-0.116) & 0.000 (-0.077) \\
        &LF 11 & 0.853 (0.209) & 0.890 (0.185) & 0.056 (-0.096) & 0.000 (-0.076) \\
        &LF 12 & 0.847 (0.204) & 0.886 (0.187) & 0.063 (-0.123) & 0.000 (-0.113) \\
        \bottomrule
    \end{tabular}
\end{table}

\begin{table}

\caption{Vision dataset raw LF performance}
   \label{tab:vision_LF}
   \centering
   \begin{tabular}{llllll}
     \toprule
    Dataset & LF & Acc & F1 & $\Delta_{DP}$ & $\Delta_{EO} $  \\
     \midrule 
     \multirow{5}{*}{CelebA} & LF 1 (ResNet-18 fine-tuned on gender classification dataset) & 0.798 & 0.794 & 0.328 & 0.284 \\
                             & LF 2 (ResNet-34 fine-tuned on FairFace dataset)& 0.890 & 0.901 &  0.314 & 0.105 \\
                             & LF 3 (ResNet-34 fine-tuned on UTKFace dataset)& 0.826 & 0.831 & 0.309 & 0.195 \\
                             & LF 4 (ResNet-34 fine-tuned on UTKFace dataset (White only))& 0.825 & 0.832 & 0.277 & 0.131 \\
                             & LF 5 (ResNet-34 fine-tuned on UTKFace dataset (non-White only))& 0.818 & 0.832& 0.271 & 0.134 \\
                             & LF 6 (ResNet-34 fine-tuned on UTKFace dataset (age $\geq 50$ only)& 0.764 & 0.750 & 0.279 & 0.194 \\
                             & LF 7 (ResNet-34 fine-tuned on UTKFace dataset (age $< 50$ only))& 0.830 & 0.845 & 0.299 & 0.175 \\
     \midrule
     \multirow{5}{*}{UTKFace} & LF 1 (ResNet-18 fine-tuned on gender classification dataset) & 0.869 & 0.856 & 0.060 & 0.039 \\
                            & LF 2 (ResNet-34 fine-tuned on gender classification dataset) & 0.854 & 0.842 & 0.060 & 0.060 \\
                            & LF 3 (ResNet-34 fine-tuned on CelebA dataset) & 0.742 & 0.758 & 0.158 & 0.032 \\
                            & LF 4 (ResNet-34 fine-tuned on CelebA dataset (attractive only)) & 0.580 & 0.692 & 0.065 & 0.002 \\
                            & LF 5 (ResNet-34 fine-tuned on CelebA dataset (non-attractive only)) & 0.687 & 0.608 & 0.129 & 0.034 \\
                            & LF 6 (ResNet-34 fine-tuned on CelebA dataset (young only)) & 0.664 & 0.729 & 0.116 & 0.012 \\
                            & LF 7 (ResNet-34 fine-tuned on CelebA dataset (non-young only))& 0.619 & 0.429 & 0.136 & 0.081 \\
                            & LF 8 (ResNet-34 fine-tuned on CelebA dataset (unfair sampling))& 0.631 & 0.676 & 0.113 & 0.053 \\
    \bottomrule
   \end{tabular}
 \end{table}

\begin{table}

\label{tab:vision_naive_LF}
\caption{Vision dataset SBM LF (w/o OT) performance. $\Delta$s are obtained by comparison with raw LF performance.}
    \centering
    \begin{tabular}{llllll}
    \toprule
        Dataset & LF & Acc ($\Delta$) & F1 ($\Delta$) & $\Delta_{DP}$ ($\Delta$) & $\Delta_{EO}$ ($\Delta$) \\ 
        \midrule
        \multirow{5}{*}{CelebA} & LF 1 & 0.847 (0.049) & 0.832 (0.038) & 0.328 (0.000) & 0.267 (-0.017) \\ 
        &LF 2 & 0.890 (0.000) & 0.895 (-0.006) & 0.314 (0.000) & 0.101 (-0.004) \\ 
        &LF 3 & 0.926 (0.100) & 0.923 (0.092) & 0.309 (0.000) & 0.097 (-0.098) \\ 
        &LF 4 & 0.914 (0.089) & 0.912 (0.080) & 0.277 (0.000) & 0.027 (-0.104) \\ 
        &LF 5 & 0.899 (0.081) & 0.900 (0.068) & 0.271 (0.000) & 0.030 (-0.104) \\ 
        &LF 6 & 0.705 (-0.059) & 0.629 (-0.121) & 0.177 (-0.102) & 0.052 (-0.142) \\
        &LF 7 & 0.913 (0.083) & 0.915 (0.070) & 0.299 (0.000) & 0.056 (-0.119) \\ 
        \midrule
        \multirow{5}{*}{UTKFace} & LF 1 & 0.929 (0.060) & 0.924 (0.068) & 0.102 (0.042) & 0.011 (-0.028) \\
        &LF 2 & 0.939 (0.085) & 0.935 (0.093) & 0.102 (0.042) & 0.007 (-0.053) \\ 
        &LF 3 & 0.631 (-0.111) & 0.678 (-0.080) & 0.078 (-0.080) & 0.034 (0.002) \\ 
        &LF 4 & 0.549 (-0.031) & 0.681 (-0.011) & 0.017 (-0.048) & 0.002 (0.000) \\ 
        &LF 5 & 0.740 (0.053) & 0.679 (0.071) & 0.129 (0.000) & 0.040 (0.006) \\ 
        &LF 6 & 0.694 (0.030) & 0.755 (0.026) & 0.116 (0.000) & 0.037 (0.025) \\ 
        &LF 7 & 0.694 (0.075) & 0.541 (0.112) & 0.061 (-0.075) & 0.033 (-0.048) \\ 
        &LF 8 & 0.591 (-0.040) & 0.654 (-0.022) & 0.071 (-0.042) & 0.054 (0.001) \\ 
        \bottomrule
    \end{tabular}
\end{table}

\begin{table}

\label{tab:vision_linear_LF}
\caption{Vision dataset SBM (OT linear) LF performance. $\Delta$s are obtained by comparison with raw LF performance.}
    \centering
    \begin{tabular}{llllll}
    \toprule
        Dataset & LF & Acc ($\Delta$) & F1 ($\Delta$) & $\Delta_{DP}$ ($\Delta$) & $\Delta_{EO}$ ($\Delta$) \\ 
        \midrule
        \multirow{5}{*}{CelebA} & LF 1 & 0.847 (0.049) & 0.832 (0.038) & 0.328 (0.000) & 0.268 (-0.016) \\
        &LF 2 & 0.890 (0.000) & 0.894 (-0.007) & 0.314 (0.000) & 0.102 (-0.003) \\ 
        &LF 3 & 0.926 (0.100) & 0.922 (0.091) & 0.309 (0.000) & 0.098 (-0.097) \\ 
        &LF 4 & 0.915 (0.090) & 0.913 (0.081) & 0.277 (0.000) & 0.029 (-0.102) \\ 
        &LF 5 & 0.898 (0.080) & 0.900 (0.068) & 0.271 (0.000) & 0.031 (-0.103) \\ 
        &LF 6 & 0.648 (-0.116) & 0.498 (-0.252) & 0.059 (-0.220) & 0.217 (0.023) \\ 
        &LF 7 & 0.914 (0.084) & 0.916 (0.071) & 0.299 (0.000) & 0.058 (-0.117) \\ 
        \midrule
        \multirow{5}{*}{UTKFace} & LF 1 & 0.931 (0.062) & 0.925 (0.069) & 0.026 (-0.034) & 0.012 (-0.027) \\ 
        & LF 2 & 0.945 (0.091) & 0.940 (0.098) & 0.017 (-0.043) & 0.006 (-0.054) \\ 
        & LF 3 & 0.599 (-0.143) & 0.667 (-0.091) & 0.004 (-0.154) & 0.001 (-0.031) \\
        &LF 4 & 0.523 (-0.057) & 0.667 (-0.025) & 0.008 (-0.057) & 0.002 (0.000) \\ 
        &LF 5 & 0.738 (0.051) & 0.674 (0.066) & 0.129 (0.000) & 0.029 (-0.005) \\ 
        &LF 6 & 0.691 (0.027) & 0.752 (0.023) & 0.116 (0.000) & 0.037 (0.025) \\ 
        &LF 7 & 0.690 (0.071) & 0.525 (0.096) & 0.000 (-0.136) & 0.016 (-0.065) \\ 
        &LF 8 & 0.572 (-0.059) & 0.655 (-0.021) & 0.001 (-0.112) & 0.014 (-0.039) \\
        \bottomrule 
    \end{tabular}
\end{table}

\begin{table}
    \caption{Vision dataset SBM (OT sinkhorn) LF performance. $\Delta$s are obtained by comparison with raw LF performance.}
    \label{tab:vision_sinkhorn_LF}
    \centering
    \begin{tabular}{llllll}
    \toprule
        Dataset & LF & Acc ($\Delta$) & F1 ($\Delta$) & $\Delta_{DP}$ ($\Delta$) & $\Delta_{EO}$ ($\Delta$) \\ 
        \midrule
        \multirow{5}{*}{CelebA} & LF 1 & 0.850 (0.052) & 0.835 (0.041) & 0.328 (0.000) & 0.266 (-0.018) \\
        &LF 2 & 0.893 (0.003) & 0.897 (-0.004) & 0.314 (0.000) & 0.101 (-0.004) \\ 
        &LF 3 & 0.923 (0.097) & 0.920 (0.089) & 0.309 (0.000) & 0.098 (-0.097) \\ 
        &LF 4 & 0.913 (0.088) & 0.910 (0.078) & 0.277 (0.000) & 0.029 (-0.102) \\ 
        &LF 5 & 0.901 (0.083) & 0.903 (0.071) & 0.271 (0.000) & 0.031 (-0.103) \\ 
        &LF 6 & 0.618 (-0.146) & 0.430 (-0.320) & 0.016 (-0.263) & 0.282 (0.088) \\ 
        &LF 7 & 0.911 (0.081) & 0.913 (0.068) & 0.299 (0.000) & 0.059 (-0.116) \\ 
        \midrule
        \multirow{5}{*}{UTKFace} &LF 1 & 0.931 (0.062) & 0.926 (0.070) & 0.010 (-0.050) & 0.001 (-0.038) \\
        &LF 2 & 0.949 (0.095) & 0.945 (0.103) & 0.015 (-0.045) & 0.001 (-0.059) \\ 
        &LF 3 & 0.577 (-0.165) & 0.652 (-0.106) & 0.003 (-0.155) & 0.013 (-0.019) \\
        &LF 4 & 0.517 (-0.063) & 0.664 (-0.028) & 0.006 (-0.059) & 0.007 (0.005) \\ 
        &LF 5 & 0.730 (0.043) & 0.669 (0.061) & 0.129 (0.000) & 0.018 (-0.016) \\ 
        &LF 6 & 0.694 (0.030) & 0.756 (0.027) & 0.116 (0.000) & 0.036 (0.024) \\ 
        &LF 7 & 0.683 (0.064) & 0.523 (0.094) & 0.010 (-0.126) & 0.007 (-0.074) \\ 
        &LF 8 & 0.562 (-0.069) & 0.652 (-0.024) & 0.009 (-0.104) & 0.012 (-0.041) \\
        \bottomrule
    \end{tabular}
\end{table}

\clearpage
\subsection{Identification of centers}
While our method improves performance by matching one group distribution and attempting to make these uniform, it does not imply accuracy improvement.
A presumption of our method is that the group with high (estimated) accuracy possesses the high accuracy regime and our method can transport data points to this high accuracy regime while keeping their structure, which results in accuracy improvements.
To empirically support this hypothesis, we used the following procedure and visualized the results in Figure \ref{fig:lf_degradation_tabular}, \ref{fig:lf_degradation_NLP datasets}, \ref{fig:lf_degradation_vision datasets}.

\begin{enumerate}
    
    \item Find the best accuracy center by evaluating the accuracy of the nearest 10\% of data points for each center candidate point.
    \item Expand 2\% percent of data points closest to the center each time, compute their accumulated average accuracy (y-axis) and the farthest distance (x-axis) from the neighborhood
    \item Find the group with better accuracy group and visualize their accumulated average accuracy (y-axis) and the farthest distance (x-axis) in each group.
\end{enumerate}

\begin{figure}

	\centering
	\subfigure [Adult (raw)]{
        \includegraphics[width=0.95\textwidth]{figures/lf_degradation_adult.pdf}}
        
        \subfigure [Bank Marketing (raw)]{
        \includegraphics[width=0.95\textwidth]{figures/lf_degradation_bank.pdf}}
\caption{Identification of high accuracy regimes for tabular datasets.}
\label{fig:lf_degradation_tabular}
\end{figure}

\begin{figure}

	\centering
	\subfigure [Adult (LIFT)]{
        \includegraphics[width=0.95\textwidth]{figures/lf_degradation_adult_lift.pdf}}
        \subfigure [Bank Marketing (LIFT)]{
        \includegraphics[width=0.95\textwidth]{figures/lf_degradation_bank_lift.pdf}}
\caption{Identification of high accuracy regimes for tabular datasets (LIFT).}
\label{fig:lf_degradation_tabular_lift}
\end{figure}

\begin{figure}

	\centering
	\subfigure [CivilComments]{
        \includegraphics[width=0.95\textwidth]{figures/lf_degradation_civilcomments.pdf}}
        \subfigure [HateXplain]{
        \includegraphics[width=0.95\textwidth]{figures/lf_degradation_hatexplain.pdf}}
\caption{Identification of high accuracy regimes for NLP datasets.}
\label{fig:lf_degradation_NLP datasets}
\end{figure}

\begin{figure}

        \subfigure [CelebA]{
        \includegraphics[width=0.95\textwidth]{figures/lf_degradation_celeba.pdf}}
        \subfigure [UTKFace]{
        \includegraphics[width=0.95\textwidth]{figures/lf_degradation_utkface.pdf}}
\caption{Identification of high accuracy regimes for vision datasets.}
\label{fig:lf_degradation_vision datasets}
\end{figure}

We are able to obtain two insights from the visualization.
First, the high accuracy regime typically exists in the group with the high estimated accuracy, which supports our hypothesis.
Thus accuracy improvement by optimal transport can be justified.
Secondly, the groups actually show the distributional difference in the input space $\mathcal{X}$. Given center points, lines in the high accuracy group start with a smaller distance to the center than the low accuracy group.

\clearpage
\subsection{Compatibility with other fair ML methods}\label{appendix_subsec:comb_others}
One advantage of our method is that we can use other successful fair ML methods in a supervised learning setting on top of SBM, since our method works in weak label sources while traditional fair ML methods work in the preprocessing/training/postprocessing steps, which are independent of the label model. To make this point, we tried traditional fair ML methods from fairlearn \citep{bird2020fairlearn} with each of WS settings. We used CorrelationRemover, ExponentiatedGradient \citep{agarwal2018reductions}, ThresholdOptimizer \citep{hardt2016equality} with the demographic parity (DP), equal opportunity (EO) as parity criteria, and accuracy as the performance criteria. The results are reported in Table \ref{tab:adult_comb_others} - \ref{tab:utkface_comb_others}. As expected, combining with other methods yields an accuracy-fairness tradeoff given weak label sources. Typically, SBM yields additional gains upon traditional fair ML methods. One another observation is that fair ML methods to modify equal opportunity typically fail to achieve the reduction of $\Delta_{EO}$. This can be interpreted as the result of the noise in the training set labels.

\begin{table}[!ht]
    \caption{SBM combined with other fair ML methods in Adult dataset}
    \label{tab:adult_comb_others}
    \centering
    \begin{tabular}{llllll}
    \toprule
        ~ & Fair ML method & Acc & F1 & $\Delta_{DP}$ & $\Delta_{EO}$ \\ \midrule
       \multirow{6}{*}{WS (Baseline)} & N/A & 0.717 & 0.587 & 0.475 & 0.325 \\ 
        ~ & correlation remover & 0.716 & 0.587 & 0.446 & 0.287 \\ 
        ~ & optimal threshold (DP) & 0.578 & 0.499 & 0.002 & 0.076 \\ 
        ~ & optimal threshold (EO) & 0.721 & 0.563 & 0.404 & 0.217 \\ 
        ~ & exponentiated gradient (DP gap = 0) & 0.582 & 0.502 & 0.002 & 0.066 \\ 
        ~ & exponentiated gradient (EO gap = 0) & 0.715 & 0.585 & 0.445 & 0.284 \\ \midrule
        \multirow{6}{*}{SBM (w/o OT)} & N/A & 0.720 & 0.592 & 0.439 & 0.273 \\
        ~ & correlation remover & 0.717 & 0.586 & 0.437 & 0.264 \\
        ~ & optimal threshold (DP) & 0.591 & 0.507 & 0.003 & 0.059 \\ 
        ~ & optimal threshold (EO) & 0.722 & 0.571 & 0.387 & 0.189 \\ 
        ~ & exponentiated gradient (DP gap = 0) & 0.693 & 0.525 & 0.014 & 0.052 \\ 
        ~ & exponentiated gradient (EO gap = 0) & 0.722 & 0.586 & 0.404 & 0.233 \\ \midrule
        \multirow{6}{*}{SBM (OT linear)} & N/A & 0.560 & 0.472 & 0.893 & 0.980 \\ ~ & correlation remover & 0.460 & 0.443 & 0.084 & 0.005 \\ 
        ~ & optimal threshold (DP) & 0.324 & 0.404 & 0.006 & 0.089 \\ 
        ~ & optimal threshold (EO) & 0.300 & 0.399 & 0.103 & 0.015 \\
        ~ & exponentiated gradient (DP gap = 0) & 0.345 & 0.414 & 0.002 & 0.016 \\ 
        ~ & exponentiated gradient (EO gap = 0) & 0.558 & 0.479 & 0.861 & 0.792 \\ \midrule
        \multirow{6}{*}{SBM (OT sinkhorn)} & N/A & 0.722 & 0.590 & 0.429 & 0.261 \\ ~ & correlation remover & 0.729 & 0.595 & 0.408 & 0.249 \\ 
        ~ & optimal threshold (DP) & 0.596 & 0.507 & 0.003 & 0.050 \\ 
        ~ & optimal threshold (EO) & 0.723 & 0.571 & 0.382 & 0.184 \\ 
        ~ & exponentiated gradient (DP gap = 0) & 0.687 & 0.527 & 0.011 & 0.045 \\ 
        ~ & exponentiated gradient (EO gap = 0) & 0.728 & 0.587 & 0.390 & 0.218 \\
        \bottomrule
    \end{tabular}
\end{table}

\begin{table}[!ht]
    \label{tab:adult(lift)_comb_others}
    \caption{SBM combined with other fair ML methods in Adult dataset (LIFT)}
    \centering
    \begin{tabular}{llllll}
    \toprule
        ~ & Fair ML method & Acc & F1 & $\Delta_{DP}$ & $\Delta_{EO}$ \\ \midrule
        \multirow{6}{*}{WS (Baseline)} & N/A & 0.711 & 0.584 & 0.449 & 0.290 \\
        ~ & correlation remover & 0.716 & 0.587 & 0.446 & 0.287 \\
        ~ & optimal threshold (DP) & 0.578 & 0.499 & 0.002 & 0.076 \\
        ~ & optimal threshold (EO) & 0.721 & 0.563 & 0.404 & 0.217 \\
        ~ & exponentiated gradient (DP gap = 0) & 0.582 & 0.502 & 0.002 & 0.066 \\ 
        ~ & exponentiated gradient (EO gap = 0) & 0.715 & 0.585 & 0.445 & 0.284 \\ \midrule
        \multirow{6}{*}{SBM (w/o OT)} & N/A & 0.704 & 0.366 & 0.032 & 0.192 \\
        ~ & correlation remover & 0.686 & 0.351 & 0.006 & 0.155 \\ 
        ~ & optimal threshold (DP) & 0.707 & 0.363 & 0.007 & 0.133 \\ 
        ~ & optimal threshold (EO) & 0.713 & 0.362 & 0.022 & 0.079 \\ 
        ~ & exponentiated gradient (DP gap = 0) & 0.682 & 0.350 & 0.011 & 0.163 \\ 
        ~ & exponentiated gradient (EO gap = 0) & 0.701 & 0.369 & 0.019 & 0.134 \\ \midrule
        \multirow{6}{*}{SBM (OT linear)} & N/A & 0.700 & 0.520 & 0.015 & 0.138 \\ 
        ~ & correlation remover & 0.686 & 0.504 & 0.011 & 0.105 \\
        ~ & optimal threshold (DP) & 0.701 & 0.520 & 0.008 & 0.124 \\
        ~ & optimal threshold (EO) & 0.712 & 0.521 & 0.060 & 0.025 \\ 
        ~ & exponentiated gradient (DP gap = 0) & 0.673 & 0.504 & 0.005 & 0.071 \\ ~ & exponentiated gradient (EO gap = 0) & 0.691 & 0.516 & 0.058 & 0.035 \\ \midrule
        \multirow{6}{*}{SBM (OT sinkhorn)} & N/A & 0.782 & 0.448 & 0.000 & 0.178 \\ 
        ~ & correlation remover & 0.772 & 0.435 & 0.002 & 0.180 \\ 
        ~ & optimal threshold (DP) & 0.782 & 0.447 & 0.001 & 0.176 \\ 
        ~ & optimal threshold (EO) & 0.790 & 0.427 & 0.087 & 0.104 \\ 
        ~ & exponentiated gradient (DP gap = 0) & 0.784 & 0.452 & 0.000 & 0.171 \\ 
        ~ & exponentiated gradient (EO gap = 0) & 0.747 & 0.380 & 0.107 & 0.049 \\
        \bottomrule
    \end{tabular}
\end{table}

\begin{table}[!ht]
\label{tab:bank_comb_others}
    \caption{SBM combined with other fair ML methods in Bank Marketing dataset}
    \centering
    \begin{tabular}{llllll}
    \toprule
        ~ & Fair ML method & Acc & F1 & $\Delta_{DP}$ & $\Delta_{EO}$ \\ \midrule
        \multirow{6}{*}{WS (Baseline)} & N/A & 0.674 & 0.258 & 0.543 & 0.450 \\ 
        ~ & correlation remover & 0.890 & 0.057 & 0.002 & 0.006 \\ 
        ~ & optimal threshold (DP) & 0.890 & 0.058 & 0.002 & 0.007 \\
        ~ & optimal threshold (EO) & 0.890 & 0.066 & 0.030 & 0.040 \\ 
        ~ & exponentiated gradient (DP gap = 0) & 0.889 & 0.039 & 0.000 & 0.009 \\ 
        ~ & exponentiated gradient (EO gap = 0) & 0.890 & 0.070 & 0.033 & 0.051 \\ \midrule
        \multirow{6}{*}{SBM (w/o OT)} & N/A & 0.876 & 0.550 & 0.106 & 0.064 \\ 
        ~ & correlation remover & 0.874 & 0.547 & 0.064 & 0.095 \\ 
        ~ & optimal threshold (DP) & 0.876 & 0.547 & 0.031 & 0.208 \\
        ~ & optimal threshold (EO) & 0.876 & 0.548 & 0.053 & 0.171 \\ 
        ~ & exponentiated gradient (DP gap = 0) & 0.877 & 0.525 & 0.037 & 0.182 \\
        ~ & exponentiated gradient (EO gap = 0) & 0.872 & 0.531 & 0.066 & 0.124 \\ \midrule
        \multirow{6}{*}{SBM (OT linear)} & N/A & 0.892 & 0.304 & 0.095 & 0.124 \\
        ~ & correlation remover & 0.890 & 0.290 & 0.011 & 0.111 \\ 
        ~ & optimal threshold (DP) & 0.891 & 0.280 & 0.008 & 0.163 \\
        ~ & optimal threshold (EO) & 0.881 & 0.313 & 0.841 & 0.678 \\ 
        ~ & exponentiated gradient (DP gap = 0) & 0.891 & 0.263 & 0.003 & 0.106 \\ 
        ~ & exponentiated gradient (EO gap = 0) & 0.895 & 0.296 & 0.097 & 0.136 \\ \midrule
        \multirow{6}{*}{SBM (OT sinkhorn)} & N/A & 0.847 & 0.515 & 0.122 & 0.080 \\ ~ & correlation remover & 0.847 & 0.512 & 0.072 & 0.122 \\
        ~ & optimal threshold (DP) & 0.846 & 0.511 & 0.043 & 0.236 \\
        ~ & optimal threshold (EO) & 0.847 & 0.515 & 0.113 & 0.104 \\
        ~ & exponentiated gradient (DP gap = 0) & 0.843 & 0.487 & 0.052 & 0.143 \\ 
        ~ & exponentiated gradient (EO gap = 0) & 0.848 & 0.512 & 0.114 & 0.088 \\
        \bottomrule
    \end{tabular}
\end{table}

\begin{table}[!ht]
\label{tab:bank(lift)_comb_others}
 \caption{SBM combined with other fair ML methods in Bank Marketing dataset (LIFT)}
    \centering
    \begin{tabular}{llllll}
    \toprule
        ~ & Fair ML method & Acc & F1 & $\Delta_{DP}$ & $\Delta_{EO}$\\ \midrule
        \multirow{6}{*}{WS (Baseline)} & N/A & 0.674 & 0.258 & 0.543 & 0.450 \\
        ~ & correlation remover & 0.890 & 0.057 & 0.002 & 0.006 \\
        ~ & optimal threshold (DP) & 0.890 & 0.058 & 0.002 & 0.007 \\
        ~ & optimal threshold (EO) & 0.890 & 0.066 & 0.030 & 0.040 \\
        ~ & exponentiated gradient (DP gap = 0) & 0.889 & 0.039 & 0.000 & 0.009 \\
        ~ & exponentiated gradient (EO gap = 0) & 0.890 & 0.070 & 0.033 & 0.051 \\ \midrule
        \multirow{6}{*}{SBM (w/o OT)} & N/A & 0.698 & 0.255 & 0.088 & 0.137 \\
        ~ & correlation remover & 0.836 & 0.358 & 0.025 & 0.114 \\
        ~ & optimal threshold (DP) & 0.699 & 0.252 & 0.002 & 0.019 \\
        ~ & optimal threshold (EO) & 0.698 & 0.253 & 0.006 & 0.028 \\
        ~ & exponentiated gradient (DP gap = 0) & 0.687 & 0.262 & 0.014 & 0.053 \\
        ~ & exponentiated gradient (EO gap = 0) & 0.654 & 0.226 & 0.096 & 0.107 \\ \midrule
        \multirow{6}{*}{SBM (OT linear)} & N/A & 0.892 & 0.305 & 0.104 & 0.121 \\
        ~ & correlation remover & 0.891 & 0.304 & 0.079 & 0.000\\
        ~ & optimal threshold (DP) & 0.891 & 0.289 & 0.016 & 0.094 \\
        ~ & optimal threshold (EO) & 0.892 & 0.305 & 0.103 & 0.121 \\
        ~ & exponentiated gradient (DP gap = 0) & 0.893 & 0.265 & 0.001 & 0.093 \\
        ~ & exponentiated gradient (EO gap = 0) & 0.892 & 0.305 & 0.100 & 0.109 \\ \midrule
        \multirow{6}{*}{SBM (OT sinkhorn)} & N/A & 0.698 & 0.080 & 0.109 & 0.072 \\
        ~ & correlation remover & 0.699 & 0.081 & 0.230 & 0.106 \\
        ~ & optimal threshold (DP) & 0.697 & 0.083 & 0.028 & 0.011 \\
        ~ & optimal threshold (EO) & 0.695 & 0.089 & 0.174 & 0.205 \\ 
        ~ & exponentiated gradient (DP gap = 0) & 0.681 & 0.113 & 0.032 & 0.063 \\ 
        ~ & exponentiated gradient (EO gap = 0) & 0.691 & 0.124 & 0.041 & 0.036 \\
        \bottomrule
    \end{tabular}
\end{table}

\begin{table}[!ht]
\label{tab:civilcomments_comb_others}
 \caption{SBM combined with other fair ML methods in CivilComments dataset}
    \centering
    \begin{tabular}{llllll}
    \toprule
        ~ & Fair ML method & Acc & F1 & $\Delta_{DP}$ & $\Delta_{EO}$\\ \midrule
        \multirow{6}{*}{WS (Baseline)} & N/A & 0.854 & 0.223 & 0.560 & 0.546 \\ 
        ~ & correlation remover & 0.886 & 0.000 & 0.000 & 0.000 \\ 
        ~ & optimal threshold (DP) & 0.886 & 0.000 & 0.000 & 0.000 \\
        ~ & optimal threshold (EO) & 0.886 & 0.000 & 0.000 & 0.000 \\
        ~ & exponentiated gradient (DP gap = 0) & 0.886 & 0.000 & 0.000 & 0.000 \\ 
        ~ & exponentiated gradient (EO gap = 0) & 0.886 & 0.000 & 0.000 & 0.000 \\ \midrule
        \multirow{6}{*}{SBM (w/o OT)} & N/A & 0.879 & 0.068 & 0.048 & 0.047 \\
        ~ & correlation remover & 0.878 & 0.062 & 0.010 & 0.030 \\ 
        ~ & optimal threshold (DP) & 0.880 & 0.054 & 0.001 & 0.015 \\
        ~ & optimal threshold (EO) & 0.880 & 0.061 & 0.019 & 0.010 \\ 
        ~ & exponentiated gradient (DP gap = 0) & 0.881 & 0.046 & 0.002 & 0.008 \\ 
        ~ & exponentiated gradient (EO gap = 0) & 0.880 & 0.059 & 0.018 & 0.010 \\ \midrule
        \multirow{6}{*}{SBM (OT linear)} & N/A & 0.880 & 0.070 & 0.042 & 0.039 \\ ~ & correlation remover & 0.879 & 0.056 & 0.011 & 0.028 \\
        ~ & optimal threshold (DP) & 0.880 & 0.060 & 0.001 & 0.017 \\
        ~ & optimal threshold (EO) & 0.880 & 0.063 & 0.013 & 0.002 \\
        ~ & exponentiated gradient (DP gap = 0) & 0.882 & 0.043 & 0.002 & 0.008 \\ 
        ~ & exponentiated gradient (EO gap = 0) & 0.882 & 0.039 & 0.006 & 0.001 \\ \midrule
        \multirow{6}{*}{SBM (OT sinkhorn)} & N/A & 0.882 & 0.047 & 0.028 & 0.026 \\ ~ & correlation remover & 0.879 & 0.057 & 0.011 & 0.029 \\ 
        ~ & optimal threshold (DP) & 0.882 & 0.040 & 0.000 & 0.011 \\
        ~ & optimal threshold (EO) & 0.882 & 0.042 & 0.010 & 0.000 \\ 
        ~ & exponentiated gradient (DP gap = 0) & 0.881 & 0.045 & 0.001 & 0.008 \\ 
        ~ & exponentiated gradient (EO gap = 0) & 0.880 & 0.056 & 0.016 & 0.005 \\ \bottomrule
    \end{tabular}
\end{table}

\begin{table}[!ht]
\label{tab:hatexplain_comb_others}
 \caption{SBM combined with other fair ML methods in HateXplain dataset}
    \centering
    \begin{tabular}{|l|l|l|l|l|l|}
    \toprule
        ~ & Fair ML method & Acc & F1 & $\Delta_{DP}$ & $\Delta_{EO}$\\ \midrule
       \multirow{6}{*}{WS (Baseline)} & N/A & 0.584 & 0.590 & 0.171 & 0.133 \\
        ~ & correlation remover & 0.555 & 0.557 & 0.007 & 0.031 \\
        ~ & optimal threshold (DP) & 0.539 & 0.515 & 0.005 & 0.047 \\ 
        ~ & optimal threshold (EO) & 0.573 & 0.573 & 0.129 & 0.090 \\
        ~ & exponentiated gradient (DP gap = 0) & 0.562 & 0.561 & 0.006 & 0.055 \\ ~ & exponentiated gradient (EO gap = 0) & 0.579 & 0.586 & 0.130 & 0.093 \\ \midrule
        \multirow{6}{*}{SBM (w/o OT)} & N/A & 0.592 & 0.637 & 0.159 & 0.138 \\
        ~ & correlation remover & 0.563 & 0.616 & 0.033 & 0.053 \\
        ~ & optimal threshold (DP) & 0.586 & 0.660 & 0.013 & 0.006 \\
        ~ & optimal threshold (EO) & 0.538 & 0.561 & 0.034 & 0.074 \\
        ~ & exponentiated gradient (DP gap = 0) & 0.581 & 0.638 & 0.039 & 0.013 \\
        ~ & exponentiated gradient (EO gap = 0) & 0.580 & 0.630 & 0.047 & 0.095 \\\midrule
        \multirow{6}{*}{SBM (OT linear)} & N/A & 0.606 & 0.670 & 0.120 & 0.101 \\ ~ & correlation remover & 0.587 & 0.657 & 0.057 & 0.087 \\
        ~ & optimal threshold (DP) & 0.600 & 0.683 & 0.010 & 0.004 \\
        ~ & optimal threshold (EO) & 0.563 & 0.615 & 0.039 & 0.071 \\ 
        ~ & exponentiated gradient (DP gap = 0) & 0.600 & 0.673 & 0.029 & 0.011 \\ 
        ~ & exponentiated gradient (EO gap = 0) & 0.593 & 0.669 & 0.044 & 0.087 \\ \midrule
        \multirow{6}{*}{SBM (OT sinkhorn)} & N/A & 0.612 & 0.687 & 0.072 & 0.037 \\ 
        ~ & correlation remover & 0.587 & 0.668 & 0.073 & 0.105 \\ 
        ~ & optimal threshold (DP) & 0.607 & 0.694 & 0.002 & 0.031 \\ 
        ~ & optimal threshold (EO) & 0.572 & 0.696 & 0.201 & 0.182 \\
        ~ & exponentiated gradient (DP gap = 0) & 0.598 & 0.683 & 0.005 & 0.020 \\ 
        ~ & exponentiated gradient (EO gap = 0) & 0.585 & 0.672 & 0.070 & 0.093 \\ \bottomrule
    \end{tabular}
\end{table}

\begin{table}[!ht]
\label{tab:celeba_comb_others}
 \caption{SBM combined with other fair ML methods in CelebA dataset}
    \centering
    \begin{tabular}{|l|l|l|l|l|l|}
    \toprule
        ~ & Fair ML method & Acc & F1 & $\Delta_{DP}$ & $\Delta_{EO}$\\ \midrule
        \multirow{6}{*}{WS (Baseline)} & N/A & 0.866 & 0.879 & 0.308 & 0.193 \\
        ~ & correlation remover & 0.845 & 0.862 & 0.099 & 0.066 \\
        ~ & optimal threshold (DP) & 0.816 & 0.845 & 0.009 & 0.035 \\
        ~ & optimal threshold (EO) & 0.789 & 0.793 & 0.196 & 0.033 \\
        ~ & exponentiated gradient (DP gap = 0) & 0.781 & 0.814 & 0.008 & 0.006 \\ 
        ~ & exponentiated gradient (EO gap = 0) & 0.838 & 0.854 & 0.205 & 0.025 \\ \midrule
       \multirow{6}{*}{SBM (w/o OT)}& N/A & 0.870 & 0.883 & 0.309 & 0.192 \\
        ~ & correlation remover & 0.849 & 0.865 & 0.095 & 0.066 \\ 
        ~ & optimal threshold (DP) & 0.819 & 0.848 & 0.009 & 0.038 \\ 
        ~ & optimal threshold (EO) & 0.792 & 0.798 & 0.194 & 0.030 \\ 
        ~ & exponentiated gradient (DP gap = 0) & 0.783 & 0.818 & 0.006 & 0.007 \\ 
        ~ & exponentiated gradient (EO gap = 0) & 0.841 & 0.857 & 0.206 & 0.029 \\ \midrule
        \multirow{6}{*}{SBM (OT linear)}& N/A & 0.870 & 0.883 & 0.306 & 0.185 \\ 
        ~ & correlation remover & 0.849 & 0.866 & 0.096 & 0.066 \\
        ~ & optimal threshold (DP) & 0.819 & 0.848 & 0.010 & 0.034 \\
        ~ & optimal threshold (EO) & 0.792 & 0.798 & 0.193 & 0.023 \\
        ~ & exponentiated gradient (DP gap = 0) & 0.783 & 0.818 & 0.007 & 0.008 \\ 
        ~ & exponentiated gradient (EO gap = 0) & 0.841 & 0.857 & 0.203 & 0.026 \\ \midrule
        \multirow{6}{*}{SBM (OT sinkhorn)} & N/A & 0.872 & 0.885 & 0.306 & 0.184 \\ ~ & correlation remover & 0.851 & 0.867 & 0.097 & 0.062 \\
        ~ & optimal threshold (DP) & 0.821 & 0.850 & 0.010 & 0.035 \\
        ~ & optimal threshold (EO) & 0.795 & 0.801 & 0.193 & 0.023 \\
        ~ & exponentiated gradient (DP gap = 0) & 0.784 & 0.819 & 0.008 & 0.010 \\
        ~ & exponentiated gradient (EO gap = 0) & 0.840 & 0.857 & 0.200 & 0.022 \\ \bottomrule
    \end{tabular}
\end{table}

\begin{table}[!ht]
 \caption{SBM combined with other fair ML methods in UTKFace dataset}
 \label{tab:utkface_comb_others}
    \centering
    \begin{tabular}{|l|l|l|l|l|l|}
    \toprule
        ~ & Fair ML method & Acc & F1 & $\Delta_{DP}$ & $\Delta_{EO}$ \\ \midrule
       \multirow{6}{*}{WS (Baseline)} & N/A & 0.791 & 0.791 & 0.172 & 0.073 \\
        ~ & correlation remover & 0.787 & 0.786 & 0.034 & 0.051 \\
        ~ & optimal threshold (DP) & 0.774 & 0.767 & 0.040 & 0.215 \\ 
        ~ & optimal threshold (EO) & 0.788 & 0.786 & 0.114 & 0.005 \\ 
        ~ & exponentiated gradient (DP gap = 0) & 0.769 & 0.762 & 0.029 & 0.078 \\ ~ & exponentiated gradient (EO gap = 0) & 0.792 & 0.790 & 0.126 & 0.026 \\ \midrule
        \multirow{6}{*}{SBM (w/o OT)} & N/A & 0.797 & 0.790 & 0.164 & 0.077 \\
        ~ & correlation remover & 0.791 & 0.793 & 0.006 & 0.091 \\ 
        ~ & optimal threshold (DP) & 0.764 & 0.791 & 0.033 & 0.202 \\
        ~ & optimal threshold (EO) & 0.789 & 0.791 & 0.165 & 0.077 \\
        ~ & exponentiated gradient (DP gap = 0) & 0.760 & 0.791 & 0.024 & 0.069 \\ 
        ~ & exponentiated gradient (EO gap = 0) & 0.791 & 0.792 & 0.158 & 0.076 \\ \midrule
        \multirow{6}{*}{SBM (OT linear)} & N/A & 0.800 & 0.793 & 0.135 & 0.043 \\ 
        ~ & correlation remover & 0.799 & 0.791 & 0.004 & 0.098 \\
        ~ & optimal threshold (DP) & 0.785 & 0.772 & 0.034 & 0.195 \\
        ~ & optimal threshold (EO) & 0.800 & 0.793 & 0.128 & 0.038 \\
        ~ & exponentiated gradient (DP gap = 0) & 0.779 & 0.764 & 0.024 & 0.069 \\ 
        ~ & exponentiated gradient (EO gap = 0) & 0.797 & 0.789 & 0.123 & 0.030 \\ \midrule
        \multirow{6}{*}{SBM (OT sinkhorn)} & N/A & 0.804 & 0.798 & 0.130 & 0.041 \\ 
        ~ & correlation remover & 0.799 & 0.794 & 0.012 & 0.087 \\
        ~ & optimal threshold (DP) & 0.789 & 0.777 & 0.036 & 0.195 \\
        ~ & optimal threshold (EO) & 0.799 & 0.794 & 0.168 & 0.046 \\
        ~ & exponentiated gradient (DP gap = 0) & 0.776 & 0.764 & 0.023 & 0.068 \\ 
        ~ & exponentiated gradient (EO gap = 0) & 0.801 & 0.796 & 0.141 & 0.044 \\ \bottomrule
    \end{tabular}
\end{table}
